# Supplementary material for: Novel approach to measure quark/gluon jets at the LHC
Source: arXiv:2307.15378 source file (2023-12-06)
Supplement: Supplementary file 1 [file appendix.tex]

\section{Appendix}
\label{sec:appendix}
\begin{figure}[h!]
    \centering
    \includegraphics[width=8cm]{./figures/delta_scatter/deltacomb_radius_lam_1.pdf} 
    \label{fig:delta_scatter_lam_1}
\end{figure}

\begin{figure}[h!]
    \centering
    \includegraphics[width=8cm]{./figures/delta_scatter/deltacomb_radius_lam_2.pdf} 
    \label{fig:delta_scatter_lam_2}
\end{figure}

\begin{figure}[h!]
    \centering
    \includegraphics[width=8cm]{./figures/delta_scatter/deltacomb_radius_lam_3.pdf} 
    \label{fig:delta_scatter_lam_3}
\end{figure}

\begin{figure}[h!]
    \centering
    \includegraphics[width=8cm]{./figures/delta_scatter/deltacomb_radius_lam_4.pdf} 
    \label{fig:delta_scatter_lam_4}
\end{figure}

\begin{figure}[h!]
    \centering
    \includegraphics[width=8cm]{./figures/delta_scatter/deltacomb_radius_lam_5.pdf} 
    \label{fig:delta_scatter_lam_5}
\end{figure}

%% Average uncertainty
\begin{figure}[h!]
    \centering
    \includegraphics[width=8cm]{./figures/delta_scatter/sumunc_radius.pdf} 
    %\caption{}
    \label{fig:sumunc_radius}
\end{figure}

%% Comparision with Radius 0.2 %%%%%%%%%%%%55
\begin{itemize}
    \item 5 - angularities $\lambda_0^0$, $\lambda_{0.5}^1$, $\lambda_1^1$, $\lambda_0^2$, $\lambda_2^1$ 
    \item 2 - quark/gluon
    \item 1 - using no trimmed jets 
    \item 2 - jet radii $R = 0.2, 0.4$
    \item 1 - average of 5 energy combinations: 900-2360, 900-7000, 900-13000, 2360-7000, 2360-13000~GeV
    \item 1 - event generators \herwig{}
    \item 1 - region - dijet average $p_{T}$ cut (Q100)
    \item 2 - MPI and ISR switched on/off
    \item 1 - gluon fraction $f(p_{T})$ 1D approach
\end{itemize}
%%% Multiplicity %%%
\begin{figure}[h!]
    \centering
    \includegraphics[width=8cm]{./figures/angs1D_filter_herwig_average_no_7000_13000/1D_X54Y52Z128W48T93R38_clone_h_no_cut_FastJets02MultLam100__herwig_average.pdf} 
    \includegraphics[width=8cm]{./figures/angs1D_filter_herwig_average_no_7000_13000/1D_X22Y117Z289W56T48R19_clone_h_no_cut_FastJets04MultLam100__herwig_average.pdf} 
    \caption{Quark and Gluon averaged angularities $\lambda_{0}^{0}$ - left R = 0.2, right R = 0.4. 
    Using \herwig{} event generator, at Q100 region, using average of 5 energy combinations 
    900-2360, 900-7000, 900-13000, 2360-7000, 2360-13000~GeV.}
    %%for now \includegraphics[width=8cm]{./figures/angs2D_filter_herwig_average_no_7000_13000/2D_20_clone_h_no_cut_FastJets04MultLam100__herwig_average.pdf} 
    %%for now \includegraphics[width=8cm]{./figures/angs2D_filter_herwig_average_no_7000_13000/2D_5_clone_h_no_cut_FastJets10MultLam100__herwig_average.pdf} 
    %%for now \caption{2D Multiplicity $R=0.4$ (left), $R=1.0$ (right).}
    \label{fig:mult1}
    \end{figure}
    
    %%% Lha %%%
    \begin{figure}[h!]
    \centering
    \includegraphics[width=8cm]{./figures/angs1D_filter_herwig_average_no_7000_13000/1D_X33Y19Z64W24T123R37_clone_h_no_cut_FastJets02LhaLam100__herwig_average.pdf} 
    \includegraphics[width=8cm]{./figures/angs1D_filter_herwig_average_no_7000_13000/1D_X18Y69Z293W27T39R9_clone_h_no_cut_FastJets04LhaLam100__herwig_average.pdf} 
    \caption{Quark and Gluon averaged angularities $\lambda_{0.5}^{1}$ - left R = 0.2, right R = 0.4. 
    Using \herwig{} event generator, at Q100 region, using average of 5 energy combinations 
    900-2360, 900-7000, 900-13000, 2360-7000, 2360-13000~GeV.}
    %%for now \includegraphics[width=8cm]{./figures/angs2D_filter_herwig_average_no_7000_13000/2D_21_clone_h_no_cut_FastJets04LhaLam100__herwig_average.pdf} 
    %%for now \includegraphics[width=8cm]{./figures/angs2D_filter_herwig_average_no_7000_13000/2D_6_clone_h_no_cut_FastJets10LhaLam100__herwig_average.pdf} 
    %%for now \caption{2D Lha $R=0.4$ (left), $R=1.0$ (right).}
    \label{fig:lha1}
    \end{figure}
    
    %%% Width %%%
    \begin{figure}[h!]
    \centering
    \includegraphics[width=8cm]{./figures/angs1D_filter_herwig_average_no_7000_13000/1D_X22Y25Z79W22T89R28_clone_h_no_cut_FastJets02WidthLam100__herwig_average.pdf} 
    \includegraphics[width=8cm]{./figures/angs1D_filter_herwig_average_no_7000_13000/1D_X14Y85Z314W27T32R9_clone_h_no_cut_FastJets04WidthLam100__herwig_average.pdf} 
    \caption{Quark and Gluon averaged angularities $\lambda_{1}^{1}$ - left R = 0.2, right R = 0.4. 
    Using \herwig{} event generator, at Q100 region, using average of 5 energy combinations 
    900-2360, 900-7000, 900-13000, 2360-7000, 2360-13000~GeV.}
    %%for now \includegraphics[width=8cm]{./figures/angs2D_filter_herwig_average_no_7000_13000/2D_15_clone_h_no_cut_FastJets04WidthLam100__herwig_average.pdf} 
    %%for now \includegraphics[width=8cm]{./figures/angs2D_filter_herwig_average_no_7000_13000/2D_4_clone_h_no_cut_FastJets10WidthLam100__herwig_average.pdf} 
    %%for now \caption{2D Width $R=0.4$ (left), $R=1.0$ (right).}
    \label{fig:width1}
    \end{figure}
    
    %%% Pt %%%
    \begin{figure}[h!]
    \centering
    \includegraphics[width=8cm]{./figures/angs1D_filter_herwig_average_no_7000_13000/1D_X61Y16Z74W32T195R43_clone_h_no_cut_FastJets02PtLam100__herwig_average.pdf} 
    \includegraphics[width=8cm]{./figures/angs1D_filter_herwig_average_no_7000_13000/1D_X63Y30Z116W35T116R30_clone_h_no_cut_FastJets04PtLam100__herwig_average.pdf} 
    \caption{Quark and Gluon averaged angularities $\lambda_{0}^{2}$ - left R = 0.2, right R = 0.4. 
    Using \herwig{} event generator, at Q100 region, using average of 5 energy combinations 
    900-2360, 900-7000, 900-13000, 2360-7000, 2360-13000~GeV.}
    %%for now \includegraphics[width=8cm]{./figures/angs2D_filter_herwig_average_no_7000_13000/2D_41_clone_h_no_cut_FastJets04PtLam100__herwig_average.pdf} 
    %%for now \includegraphics[width=8cm]{./figures/angs2D_filter_herwig_average_no_7000_13000/2D_11_clone_h_no_cut_FastJets10PtLam100__herwig_average.pdf} 
    %%for now \caption{2D Pt $R=0.4$ (left), $R=1.0$ (right).}
    \label{fig:pt1}
    \end{figure}
    
    %%% Mass %%%
    \begin{figure}[h!]
    \centering
    \includegraphics[width=8cm]{./figures/angs1D_filter_herwig_average_no_7000_13000/1D_X23Y19Z78W21T107R26_clone_h_no_cut_FastJets02MassLam100__herwig_average.pdf} 
    \includegraphics[width=8cm]{./figures/angs1D_filter_herwig_average_no_7000_13000/1D_X9Y82Z281W26T32R9_clone_h_no_cut_FastJets04MassLam100__herwig_average.pdf} 
    \caption{Quark and Gluon averaged angularities $\lambda_{2}^{1}$ - left R = 0.2, right R = 0.4. 
    Using \herwig{} event generator, at Q100 region, using average of 5 energy combinations 
    900-2360, 900-7000, 900-13000, 2360-7000, 2360-13000~GeV.}
    %%for now \includegraphics[width=8cm]{./figures/angs2D_filter_herwig_average_no_7000_13000/2D_9_clone_h_no_cut_FastJets04MassLam100__herwig_average.pdf} 
    %%for now \includegraphics[width=8cm]{./figures/angs2D_filter_herwig_average_no_7000_13000/2D_3_clone_h_no_cut_FastJets10MassLam100__herwig_average.pdf} 
    %%for now \caption{2D Mass $R=0.4$ (left), $R=1.0$ (right).}
    \label{fig:mass1}
    \end{figure}

Plots in the Appendix shows all six energy combinations also with 7000-13000~GeV which increses statistical uncertainties.
\subsection{\herwig{} 1D Approach, Six Enerrgy Variations, Q100}
\begin{itemize}
    \item 5 - angularities $\lambda_0^0$, $\lambda_{0.5}^1$, $\lambda_1^1$, $\lambda_0^2$, $\lambda_2^1$ 
    \item 2 - quark/gluon
    \item 1 - using no trimmed jets 
    \item 2 - jet radii $R = 0.4, 1.0$
    \item 1 - average of 6 energy combinations: 900-2360, 900-7000, 900-13000, 2360-7000, 2360-13000, 7000-13000~GeV
    \item 1 - event generators \herwig{}
    \item 1 - region - dijet average $p_{T}$ cut (Q100)
    \item 2 - MPI and ISR switched on/off
    \item 1 - gluon fraction $f(p_{T})$ 1D approach
\end{itemize}

%%% Multiplicity %%%
\begin{figure}[h!]
    \centering
    \includegraphics[width=8cm]{./figures/angs1D_filter_herwig_average/1D_X19Y41Z160W58T141R37_clone_h_no_cut_FastJets04MultLam100__herwig_average.pdf} 
    \includegraphics[width=8cm]{./figures/angs1D_filter_herwig_average/1D_X5Y303Z530W66T22R12_clone_h_no_cut_FastJets10MultLam100__herwig_average.pdf} 
    \caption{Quark and Gluon averaged angularities $\lambda_{0}^{0}$ - left R = 0.4, right R = 1.0. 
    Using \herwig{} event generator, at Q100 region, using average of 6 energy combinations 
    900-2360, 900-7000, 900-13000, 2360-7000, 2360-13000, 7000-13000~GeV.}
    \label{fig:mult2}
    %%for now \includegraphics[width=8cm]{./figures/angs2D_filter_herwig_average/2D_X17Y30Z175_clone_h_no_cut_FastJets04MultLam100__herwig_average.pdf} 
    %%for now \includegraphics[width=8cm]{./figures/angs2D_filter_herwig_average/2D_X5Y305Z679_clone_h_no_cut_FastJets10MultLam100__herwig_average.pdf} 
    %%for now \caption{2D Multiplicity $R=0.4$ (left), $R=1.0$ (right).}
    \end{figure}
    
    %%% Lha %%%
    \begin{figure}[h!]
    \centering
    \includegraphics[width=8cm]{./figures/angs1D_filter_herwig_average/1D_X11Y21Z182W32T156R18_clone_h_no_cut_FastJets04LhaLam100__herwig_average.pdf} 
    \includegraphics[width=8cm]{./figures/angs1D_filter_herwig_average/1D_X5Y114Z278W45T40R16_clone_h_no_cut_FastJets10LhaLam100__herwig_average.pdf} 
    \caption{Quark and Gluon averaged angularities $\lambda_{0.5}^{1}$ - left R = 0.4, right R = 1.0. 
    Using \herwig{} event generator, at Q100 region, using average of 6 energy combinations 
    900-2360, 900-7000, 900-13000, 2360-7000, 2360-13000, 7000-13000~GeV.}
    \label{fig:lha2}

    %%for now \includegraphics[width=8cm]{./figures/angs2D_filter_herwig_average/2D_X13Y16Z91_clone_h_no_cut_FastJets04LhaLam100__herwig_average.pdf} 
    %%for now \includegraphics[width=8cm]{./figures/angs2D_filter_herwig_average/2D_X5Y81Z284_clone_h_no_cut_FastJets10LhaLam100__herwig_average.pdf} 
    %%for now \caption{2D Lha $R=0.4$ (left), $R=1.0$ (right).}
    \end{figure}
    
    %%% Width %%%
    \begin{figure}[h!]
    \centering
    \includegraphics[width=8cm]{./figures/angs1D_filter_herwig_average/1D_X9Y23Z115W33T145R29_clone_h_no_cut_FastJets04WidthLam100__herwig_average.pdf} 
    \includegraphics[width=8cm]{./figures/angs1D_filter_herwig_average/1D_X4Y122Z280W51T42R18_clone_h_no_cut_FastJets10WidthLam100__herwig_average.pdf} 
    \caption{Quark and Gluon averaged angularities $\lambda_{1}^{1}$ - left R = 0.4, right R = 1.0. 
    Using \herwig{} event generator, at Q100 region, using average of 6 energy combinations 
    900-2360, 900-7000, 900-13000, 2360-7000, 2360-13000, 7000-13000~GeV.}
    \label{fig:width2}

    %%for now \includegraphics[width=8cm]{./figures/angs2D_filter_herwig_average/2D_X11Y17Z92_clone_h_no_cut_FastJets04WidthLam100__herwig_average.pdf} 
    %%for now \includegraphics[width=8cm]{./figures/angs2D_filter_herwig_average/2D_X4Y83Z285_clone_h_no_cut_FastJets10WidthLam100__herwig_average.pdf} 
    %%for now \caption{2D Width $R=0.4$ (left), $R=1.0$ (right).}
    \end{figure}
    
    %%% Pt %%%
    \begin{figure}[h!]
    \centering
    \includegraphics[width=8cm]{./figures/angs1D_filter_herwig_average/1D_X32Y14Z47W39T279R82_clone_h_no_cut_FastJets04PtLam100__herwig_average.pdf} 
    \includegraphics[width=8cm]{./figures/angs1D_filter_herwig_average/1D_X11Y60Z112W44T74R39_clone_h_no_cut_FastJets10PtLam100__herwig_average.pdf} 
    \caption{Quark and Gluon averaged angularities $\lambda_{0}^{2}$ - left R = 0.4, right R = 1.0. 
    Using \herwig{} event generator, at Q100 region, using average of 6 energy combinations 
    900-2360, 900-7000, 900-13000, 2360-7000, 2360-13000, 7000-13000~GeV.}
    \label{fig:pt2}
    %%for now \includegraphics[width=8cm]{./figures/angs2D_filter_herwig_average/2D_X42Y9Z38_clone_h_no_cut_FastJets04PtLam100__herwig_average.pdf} 
    %%for now \includegraphics[width=8cm]{./figures/angs2D_filter_herwig_average/2D_X11Y32Z84_clone_h_no_cut_FastJets10PtLam100__herwig_average.pdf} 
    %%for now \caption{2D Pt $R=0.4$ (left), $R=1.0$ (right).}
    \end{figure}
    
    %%% Mass %%%
    \begin{figure}[h!]
    \centering
    \includegraphics[width=8cm]{./figures/angs1D_filter_herwig_average/1D_X6Y27Z105W33T122R31_clone_h_no_cut_FastJets04MassLam100__herwig_average.pdf} 
    \includegraphics[width=8cm]{./figures/angs1D_filter_herwig_average/1D_X3Y112Z253W58T52R23_clone_h_no_cut_FastJets10MassLam100__herwig_average.pdf} 
    \caption{Quark and Gluon averaged angularities $\lambda_{2}^{1}$ - left R = 0.4, right R = 1.0. 
    Using \herwig{} event generator, at Q100 region, using average of 6 energy combinations 
    900-2360, 900-7000, 900-13000, 2360-7000, 2360-13000, 7000-13000~GeV.}
    \label{fig:mass2}
    %%for now \includegraphics[width=8cm]{./figures/angs2D_filter_herwig_average/2D_X7Y18Z101_clone_h_no_cut_FastJets04MassLam100__herwig_average.pdf} 
    %%for now \includegraphics[width=8cm]{./figures/angs2D_filter_herwig_average/2D_X3Y72Z270_clone_h_no_cut_FastJets10MassLam100__herwig_average.pdf} 
    %%for now \caption{2D Mass $R=0.4$ (left), $R=1.0$ (right).}
    \end{figure}
    \clearpage
%%%%%%%%%%%%%%%%%%PYTHIA RESULTS %%%%%%%%%%%%%%%%%%%%%%%%%%%%%%%%%%
\subsection{\pythia{} 1D Approach, Six Enerrgy Variations, Q100}
\begin{itemize}
    \item 5 - angularities $\lambda_0^0$, $\lambda_{0.5}^1$, $\lambda_1^1$, $\lambda_0^2$, $\lambda_2^1$ 
    \item 2 - quark/gluon
    \item 1 - using no trimmed jets 
    \item 2 - jet radii $R = 0.4, 1.0$
    \item 1 - average of 6 energy combinations: 900-2360, 900-7000, 900-13000, 2360-7000, 2360-13000, 7000-13000~GeV
    \item 1 - event generators \pythia{}
    \item 1 - region - dijet average $p_{T}$ cut (Q100)
    \item 2 - MPI and ISR switched on/off
    \item 1 - gluon fraction $f(p_{T})$ 1D approach
\end{itemize}

%%% Multiplicity %%%
\begin{figure}[h!]
    \centering
    \includegraphics[width=8cm]{./figures/angs1D_filter_herwig_average/1D_X7Y129Z285W60T47R21_clone_h_no_cut_FastJets04MultLam100__pythia_average.pdf} 
    \includegraphics[width=8cm]{./figures/angs1D_filter_herwig_average/1D_X1Y1777Z4172W69T4R2_clone_h_no_cut_FastJets10MultLam100__pythia_average.pdf} 
    \caption{Quark and Gluon averaged angularities $\lambda_{0}^{0}$ - left R = 0.4, right R = 1.0. 
    Using \pythia{} event generator, at Q100 region, using average of 6 energy combinations 
    900-2360, 900-7000, 900-13000, 2360-7000, 2360-13000, 7000-13000~GeV.}
    \label{fig:mult2_pyt}
    %%for now \includegraphics[width=8cm]{./figures/angs2D_filter_herwig_average/2D_17_clone_h_no_cut_FastJets04MultLam100__pythia_average.pdf} 
    %%for now \includegraphics[width=8cm]{./figures/angs2D_filter_herwig_average/2D_5_clone_h_no_cut_FastJets10MultLam100__pythia_average.pdf} 
    %%for now \caption{2D Multiplicity $R=0.4$ (left), $R=1.0$ (right).}
    \end{figure}
    
    %%% Lha %%%
    \begin{figure}[h!]
    \centering
    \includegraphics[width=8cm]{./figures/angs1D_filter_herwig_average/1D_X12Y35Z148W34T98R23_clone_h_no_cut_FastJets04LhaLam100__pythia_average.pdf} 
    \includegraphics[width=8cm]{./figures/angs1D_filter_herwig_average/1D_X3Y566Z1563W52T9R3_clone_h_no_cut_FastJets10LhaLam100__pythia_average.pdf} 
    \caption{Quark and Gluon averaged angularities $\lambda_{0.5}^{1}$ - left R = 0.4, right R = 1.0. 
    Using \pythia{} event generator, at Q100 region, using average of 6 energy combinations 
    900-2360, 900-7000, 900-13000, 2360-7000, 2360-13000, 7000-13000~GeV.}
    \label{fig:lha2_pyt}

    %%for now \includegraphics[width=8cm]{./figures/angs2D_filter_herwig_average/2D_13_clone_h_no_cut_FastJets04LhaLam100__pythia_average.pdf} 
    %%for now \includegraphics[width=8cm]{./figures/angs2D_filter_herwig_average/2D_5_clone_h_no_cut_FastJets10LhaLam100__pythia_average.pdf} 
    %%for now \caption{2D Lha $R=0.4$ (left), $R=1.0$ (right).}
    \end{figure}
    
    %%% Width %%%
    \begin{figure}[h!]
    \centering
    \includegraphics[width=8cm]{./figures/angs1D_filter_herwig_average/1D_X10Y45Z205W33T74R16_clone_h_no_cut_FastJets04WidthLam100__pythia_average.pdf} 
    \includegraphics[width=8cm]{./figures/angs1D_filter_herwig_average/1D_X2Y588Z1545W59T10R4_clone_h_no_cut_FastJets10WidthLam100__pythia_average.pdf} 
    \caption{Quark and Gluon averaged angularities $\lambda_{1}^{1}$ - left R = 0.4, right R = 1.0. 
    Using \pythia{} event generator, at Q100 region, using average of 6 energy combinations 
    900-2360, 900-7000, 900-13000, 2360-7000, 2360-13000, 7000-13000~GeV.}
    \label{fig:width2_pyt}

    %%for now \includegraphics[width=8cm]{./figures/angs2D_filter_herwig_average/2D_11_clone_h_no_cut_FastJets04WidthLam100__pythia_average.pdf} 
    %%for now \includegraphics[width=8cm]{./figures/angs2D_filter_herwig_average/2D_4_clone_h_no_cut_FastJets10WidthLam100__pythia_average.pdf} 
    %%for now \caption{2D Width $R=0.4$ (left), $R=1.0$ (right).}
    \end{figure}
    
    %%% Pt %%%
    \begin{figure}[h!]
    \centering
    \includegraphics[width=8cm]{./figures/angs1D_filter_herwig_average/1D_X30Y22Z66W42T188R63_clone_h_no_cut_FastJets04PtLam100__pythia_average.pdf} 
    \includegraphics[width=8cm]{./figures/angs1D_filter_herwig_average/1D_X5Y172Z414W49T28R12_clone_h_no_cut_FastJets10PtLam100__pythia_average.pdf} 
    \caption{Quark and Gluon averaged angularities $\lambda_{0}^{2}$ - left R = 0.4, right R = 1.0. 
    Using \pythia{} event generator, at Q100 region, using average of 6 energy combinations 
    900-2360, 900-7000, 900-13000, 2360-7000, 2360-13000, 7000-13000~GeV.}
    \label{fig:pt2_pyt}
    %%for now \includegraphics[width=8cm]{./figures/angs2D_filter_herwig_average/2D_42_clone_h_no_cut_FastJets04PtLam100__pythia_average.pdf} 
    %%for now \includegraphics[width=8cm]{./figures/angs2D_filter_herwig_average/2D_11_clone_h_no_cut_FastJets10PtLam100__pythia_average.pdf} 
    %%for now \caption{2D Pt $R=0.4$ (left), $R=1.0$ (right).}
    \end{figure}
    
    %%% Mass %%%
    \begin{figure}[h!]
    \centering
    \includegraphics[width=8cm]{./figures/angs1D_filter_herwig_average/1D_X7Y52Z195W33T63R17_clone_h_no_cut_FastJets04MassLam100__pythia_average.pdf} 
    \includegraphics[width=8cm]{./figures/angs1D_filter_herwig_average/1D_X1Y704Z1555W64T9R4_clone_h_no_cut_FastJets10MassLam100__pythia_average.pdf} 
    \caption{Quark and Gluon averaged angularities $\lambda_{2}^{1}$ - left R = 0.4, right R = 1.0. 
    Using \pythia{} event generator, at Q100 region, using average of 6 energy combinations 
    900-2360, 900-7000, 900-13000, 2360-7000, 2360-13000, 7000-13000~GeV.}
    \label{fig:mass2_pyt}
    %%for now \includegraphics[width=8cm]{./figures/angs2D_filter_herwig_average/2D_X7Y44Z169_clone_h_no_cut_FastJets04MassLam100__pythia_average.pdf} 
    %%for now \includegraphics[width=8cm]{./figures/angs2D_filter_herwig_average/2D_3_clone_h_no_cut_FastJets10MassLam100__pythia_average.pdf} 
    %%for now \caption{2D Mass $R=0.4$ (left), $R=1.0$ (right).}
    \end{figure}
    \clearpage
%%%% 2D APPROACH%%%%%%%%%%%%%%%%%%%%%%%%%%%
\subsection{\herwig{} 2D Approach, Six Enerrgy Variations, Q100}
\begin{itemize}
    \item 5 - angularities $\lambda_0^0$, $\lambda_{0.5}^1$, $\lambda_1^1$, $\lambda_0^2$, $\lambda_2^1$ 
    \item 2 - quark/gluon
    \item 1 - using no trimmed jets 
    \item 2 - jet radii $R = 0.4, 1.0$
    \item 1 - average of 6 energy combinations: 900-2360, 900-7000, 900-13000, 2360-7000, 2360-13000, 7000-13000~GeV
    \item 1 - event generators \herwig{}
    \item 1 - region - dijet average $p_{T}$ cut (Q100)
    \item 2 - MPI and ISR switched on/off
    \item 1 - gluon fraction $f(p_{T})$ 2D approach
\end{itemize}

%%% Multiplicity %%%
\begin{figure}[h!]
    \centering
    \includegraphics[width=8cm]{./figures/angs2D_filter_herwig_average/2D_X17Y30Z175_clone_h_no_cut_FastJets04MultLam100__herwig_average.pdf} 
    \includegraphics[width=8cm]{./figures/angs2D_filter_herwig_average/2D_X5Y305Z679_clone_h_no_cut_FastJets10MultLam100__herwig_average.pdf} 
    \caption{Quark and Gluon averaged angularities $\lambda_{0}^{0}$ - left R = 0.4, right R = 1.0. 
    Using \herwig{} event generator, at Q100 region, using average of 6 energy combinations 
    900-2360, 900-7000, 900-13000, 2360-7000, 2360-13000, 7000-13000~GeV.}
    \label{fig:2D_mult2}
    %%for now \includegraphics[width=8cm]{./figures/angs2D_filter_herwig_average/2D_X17Y30Z175_clone_h_no_cut_FastJets04MultLam100__herwig_average.pdf} 
    %%for now \includegraphics[width=8cm]{./figures/angs2D_filter_herwig_average/2D_X5Y305Z679_clone_h_no_cut_FastJets10MultLam100__herwig_average.pdf} 
    %%for now \caption{2D Multiplicity $R=0.4$ (left), $R=1.0$ (right).}
    \end{figure}
    
    %%% Lha %%%
    \begin{figure}[h!]
    \centering
    \includegraphics[width=8cm]{./figures/angs2D_filter_herwig_average/2D_X13Y16Z91_clone_h_no_cut_FastJets04LhaLam100__herwig_average.pdf} 
    \includegraphics[width=8cm]{./figures/angs2D_filter_herwig_average/2D_X5Y81Z284_clone_h_no_cut_FastJets10LhaLam100__herwig_average.pdf} 
    \caption{Quark and Gluon averaged angularities $\lambda_{0.5}^{1}$ - left R = 0.4, right R = 1.0. 
    Using \herwig{} event generator, at Q100 region, using average of 6 energy combinations 
    900-2360, 900-7000, 900-13000, 2360-7000, 2360-13000, 7000-13000~GeV.}
    \label{fig:2D_lha2}

    %%for now \includegraphics[width=8cm]{./figures/angs2D_filter_herwig_average/2D_X13Y16Z91_clone_h_no_cut_FastJets04LhaLam100__herwig_average.pdf} 
    %%for now \includegraphics[width=8cm]{./figures/angs2D_filter_herwig_average/2D_X5Y81Z284_clone_h_no_cut_FastJets10LhaLam100__herwig_average.pdf} 
    %%for now \caption{2D Lha $R=0.4$ (left), $R=1.0$ (right).}
    \end{figure}
    
    %%% Width %%%
    \begin{figure}[h!]
    \centering
    \includegraphics[width=8cm]{./figures/angs2D_filter_herwig_average/2D_X11Y17Z92_clone_h_no_cut_FastJets04WidthLam100__herwig_average.pdf} 
    \includegraphics[width=8cm]{./figures/angs2D_filter_herwig_average/2D_X4Y83Z285_clone_h_no_cut_FastJets10WidthLam100__herwig_average.pdf} 
    \caption{Quark and Gluon averaged angularities $\lambda_{1}^{1}$ - left R = 0.4, right R = 1.0. 
    Using \herwig{} event generator, at Q100 region, using average of 6 energy combinations 
    900-2360, 900-7000, 900-13000, 2360-7000, 2360-13000, 7000-13000~GeV.}
    \label{fig:2D_width2}

    %%for now \includegraphics[width=8cm]{./figures/angs2D_filter_herwig_average/2D_X11Y17Z92_clone_h_no_cut_FastJets04WidthLam100__herwig_average.pdf} 
    %%for now \includegraphics[width=8cm]{./figures/angs2D_filter_herwig_average/2D_X4Y83Z285_clone_h_no_cut_FastJets10WidthLam100__herwig_average.pdf} 
    %%for now \caption{2D Width $R=0.4$ (left), $R=1.0$ (right).}
    \end{figure}
    
    %%% Pt %%%
    \begin{figure}[h!]
    \centering
    \includegraphics[width=8cm]{./figures/angs2D_filter_herwig_average/2D_X42Y9Z38_clone_h_no_cut_FastJets04PtLam100__herwig_average.pdf} 
    \includegraphics[width=8cm]{./figures/angs2D_filter_herwig_average/2D_X11Y32Z84_clone_h_no_cut_FastJets10PtLam100__herwig_average.pdf} 
    \caption{Quark and Gluon averaged angularities $\lambda_{0}^{2}$ - left R = 0.4, right R = 1.0. 
    Using \herwig{} event generator, at Q100 region, using average of 6 energy combinations 
    900-2360, 900-7000, 900-13000, 2360-7000, 2360-13000, 7000-13000~GeV.}
    \label{fig:2D_pt2}
    %%for now \includegraphics[width=8cm]{./figures/angs2D_filter_herwig_average/2D_X42Y9Z38_clone_h_no_cut_FastJets04PtLam100__herwig_average.pdf} 
    %%for now \includegraphics[width=8cm]{./figures/angs2D_filter_herwig_average/2D_X11Y32Z84_clone_h_no_cut_FastJets10PtLam100__herwig_average.pdf} 
    %%for now \caption{2D Pt $R=0.4$ (left), $R=1.0$ (right).}
    \end{figure}
    
    %%% Mass %%%
    \begin{figure}[h!]
    \centering
    \includegraphics[width=8cm]{./figures/angs2D_filter_herwig_average/2D_X7Y18Z101_clone_h_no_cut_FastJets04MassLam100__herwig_average.pdf} 
    \includegraphics[width=8cm]{./figures/angs2D_filter_herwig_average/2D_X3Y72Z270_clone_h_no_cut_FastJets10MassLam100__herwig_average.pdf} 
    \caption{Quark and Gluon averaged angularities $\lambda_{2}^{1}$ - left R = 0.4, right R = 1.0. 
    Using \herwig{} event generator, at Q100 region, using average of 6 energy combinations 
    900-2360, 900-7000, 900-13000, 2360-7000, 2360-13000, 7000-13000~GeV.}
    \label{fig:2D_mass2}
    %%for now \includegraphics[width=8cm]{./figures/angs2D_filter_herwig_average/2D_X7Y18Z101_clone_h_no_cut_FastJets04MassLam100__herwig_average.pdf} 
    %%for now \includegraphics[width=8cm]{./figures/angs2D_filter_herwig_average/2D_X3Y72Z270_clone_h_no_cut_FastJets10MassLam100__herwig_average.pdf} 
    %%for now \caption{2D Mass $R=0.4$ (left), $R=1.0$ (right).}
    \end{figure}
    \clearpage
%%%%%%%%%%%%%%%%%%PYTHIA RESULTS %%%%%%%%%%%%%%%%%%%%%%%%%%%%%%%%%%
\subsection{\pythia{} 2D Approach, Six Enerrgy Variations, Q100}
\begin{itemize}
    \item 5 - angularities $\lambda_0^0$, $\lambda_{0.5}^1$, $\lambda_1^1$, $\lambda_0^2$, $\lambda_2^1$ 
    \item 2 - quark/gluon
    \item 1 - using no trimmed jets 
    \item 2 - jet radii $R = 0.4, 1.0$
    \item 1 - average of 6 energy combinations: 900-2360, 900-7000, 900-13000, 2360-7000, 2360-13000, 7000-13000~GeV
    \item 1 - event generators \pythia{}
    \item 1 - region - dijet average $p_{T}$ cut (Q100)
    \item 2 - MPI and ISR switched on/off
    \item 1 - gluon fraction $f(p_{T})$ 2D approach
\end{itemize}

%%% Multiplicity %%%
\begin{figure}[h!]
    \centering
    \includegraphics[width=8cm]{./figures/angs2D_filter_herwig_average/2D_X6Y99Z259_clone_h_no_cut_FastJets04MultLam100__pythia_average.pdf} 
    \includegraphics[width=8cm]{./figures/angs2D_filter_herwig_average/2D_X1Y1121Z2901_clone_h_no_cut_FastJets10MultLam100__pythia_average.pdf} 
    \caption{Quark and Gluon averaged angularities $\lambda_{0}^{0}$ - left R = 0.4, right R = 1.0. 
    Using \pythia{} event generator, at Q100 region, using average of 6 energy combinations 
    900-2360, 900-7000, 900-13000, 2360-7000, 2360-13000, 7000-13000~GeV.}
    \label{fig:2D_mult2_pyt}
    %%for now \includegraphics[width=8cm]{./figures/angs2D_filter_herwig_average/2D_17_clone_h_no_cut_FastJets04MultLam100__pythia_average.pdf} 
    %%for now \includegraphics[width=8cm]{./figures/angs2D_filter_herwig_average/2D_5_clone_h_no_cut_FastJets10MultLam100__pythia_average.pdf} 
    %%for now \caption{2D Multiplicity $R=0.4$ (left), $R=1.0$ (right).}
    \end{figure}
    
    %%% Lha %%%
    \begin{figure}[h!]
    \centering
    \includegraphics[width=8cm]{./figures/angs2D_filter_herwig_average/2D_X13Y30Z177_clone_h_no_cut_FastJets04LhaLam100__pythia_average.pdf} 
    \includegraphics[width=8cm]{./figures/angs2D_filter_herwig_average/2D_X2Y322Z1179_clone_h_no_cut_FastJets10LhaLam100__pythia_average.pdf} 
    \caption{Quark and Gluon averaged angularities $\lambda_{0.5}^{1}$ - left R = 0.4, right R = 1.0. 
    Using \pythia{} event generator, at Q100 region, using average of 6 energy combinations 
    900-2360, 900-7000, 900-13000, 2360-7000, 2360-13000, 7000-13000~GeV.}
    \label{fig:2D_lha2_pyt}

    %%for now \includegraphics[width=8cm]{./figures/angs2D_filter_herwig_average/2D_13_clone_h_no_cut_FastJets04LhaLam100__pythia_average.pdf} 
    %%for now \includegraphics[width=8cm]{./figures/angs2D_filter_herwig_average/2D_5_clone_h_no_cut_FastJets10LhaLam100__pythia_average.pdf} 
    %%for now \caption{2D Lha $R=0.4$ (left), $R=1.0$ (right).}
    \end{figure}
    
    %%% Width %%%
    \begin{figure}[h!]
    \centering
    \includegraphics[width=8cm]{./figures/angs2D_filter_herwig_average/2D_X10Y37Z174_clone_h_no_cut_FastJets04WidthLam100__pythia_average.pdf} 
    \includegraphics[width=8cm]{./figures/angs2D_filter_herwig_average/2D_X2Y372Z1232_clone_h_no_cut_FastJets10WidthLam100__pythia_average.pdf} 
    \caption{Quark and Gluon averaged angularities $\lambda_{1}^{1}$ - left R = 0.4, right R = 1.0. 
    Using \pythia{} event generator, at Q100 region, using average of 6 energy combinations 
    900-2360, 900-7000, 900-13000, 2360-7000, 2360-13000, 7000-13000~GeV.}
    \label{fig:2D_width2_pyt}

    %%for now \includegraphics[width=8cm]{./figures/angs2D_filter_herwig_average/2D_11_clone_h_no_cut_FastJets04WidthLam100__pythia_average.pdf} 
    %%for now \includegraphics[width=8cm]{./figures/angs2D_filter_herwig_average/2D_4_clone_h_no_cut_FastJets10WidthLam100__pythia_average.pdf} 
    %%for now \caption{2D Width $R=0.4$ (left), $R=1.0$ (right).}
    \end{figure}
    
    %%% Pt %%%
    \begin{figure}[h!]
    \centering
    \includegraphics[width=8cm]{./figures/angs2D_filter_herwig_average/2D_X17Y16Z51_clone_h_no_cut_FastJets04PtLam100__pythia_average.pdf} 
    \includegraphics[width=8cm]{./figures/angs2D_filter_herwig_average/2D_X4Y77Z269_clone_h_no_cut_FastJets10PtLam100__pythia_average.pdf} 
    \caption{Quark and Gluon averaged angularities $\lambda_{0}^{2}$ - left R = 0.4, right R = 1.0. 
    Using \pythia{} event generator, at Q100 region, using average of 6 energy combinations 
    900-2360, 900-7000, 900-13000, 2360-7000, 2360-13000, 7000-13000~GeV.}
    \label{fig:2D_pt2_pyt}
    %%for now \includegraphics[width=8cm]{./figures/angs2D_filter_herwig_average/2D_42_clone_h_no_cut_FastJets04PtLam100__pythia_average.pdf} 
    %%for now \includegraphics[width=8cm]{./figures/angs2D_filter_herwig_average/2D_11_clone_h_no_cut_FastJets10PtLam100__pythia_average.pdf} 
    %%for now \caption{2D Pt $R=0.4$ (left), $R=1.0$ (right).}
    \end{figure}
    
    %%% Mass %%%
    \begin{figure}[h!]
    \centering
    \includegraphics[width=8cm]{./figures/angs2D_filter_herwig_average/2D_X7Y44Z169_clone_h_no_cut_FastJets04MassLam100__pythia_average.pdf} 
    \includegraphics[width=8cm]{./figures/angs2D_filter_herwig_average/2D_X1Y526Z1328_clone_h_no_cut_FastJets10MassLam100__pythia_average.pdf} 
    \caption{Quark and Gluon averaged angularities $\lambda_{2}^{1}$ - left R = 0.4, right R = 1.0. 
    Using \pythia{} event generator, at Q100 region, using average of 6 energy combinations 
    900-2360, 900-7000, 900-13000, 2360-7000, 2360-13000, 7000-13000~GeV.}
    \label{fig:2D_mass2_pyt}
    %%for now \includegraphics[width=8cm]{./figures/angs2D_filter_herwig_average/2D_X7Y44Z169_clone_h_no_cut_FastJets04MassLam100__pythia_average.pdf} 
    %%for now \includegraphics[width=8cm]{./figures/angs2D_filter_herwig_average/2D_3_clone_h_no_cut_FastJets10MassLam100__pythia_average.pdf} 
    %%for now \caption{2D Mass $R=0.4$ (left), $R=1.0$ (right).}
    \end{figure}
    \clearpage

    \subsection{\herwig{} 1D Approach, Six Enerrgy Variations, Q100, Trimmed Jets}
    \begin{itemize}
        \item 5 - angularities $\lambda_0^0$, $\lambda_{0.5}^1$, $\lambda_1^1$, $\lambda_0^2$, $\lambda_2^1$ 
        \item 2 - quark/gluon
        \item 1 - using trimmed jets 
        \item 2 - jet radii $R = 0.4, 1.0$
        \item 1 - average of 6 energy combinations: 900-2360, 900-7000, 900-13000, 2360-7000, 2360-13000, 7000-13000~GeV
        \item 1 - event generators \herwig{}
        \item 1 - region - dijet average $p_{T}$ cut (Q100)
        \item 2 - MPI and ISR switched on/off
        \item 1 - gluon fraction $f(p_{T})$ 1D approach
    \end{itemize}

    %%% Multiplicity %%%
    \begin{figure}[h!]
        \centering
        \includegraphics[width=8cm]{./figures/angs1D_filter_herwig_average/1D_X31Y33Z115W21T63R18_clone_h_no_cut_mmdt_FastJets04MultLam100__herwig_average.pdf} 
        \includegraphics[width=8cm]{./figures/angs1D_filter_herwig_average/1D_X8Y169Z411W24T14R6_clone_h_no_cut_mmdt_FastJets10MultLam100__herwig_average.pdf} 
        \caption{Quark and Gluon averaged angularities $\lambda_{0}^{0}$ - left R = 0.4, right R = 1.0. 
        Using \herwig{} event generator, at Q100 region, using average of 6 energy combinations 
        900-2360, 900-7000, 900-13000, 2360-7000, 2360-13000, 7000-13000~GeV.}
        \label{fig:mmdt_mult2}
        %%for now \includegraphics[width=8cm]{./figures/angs2D_filter_herwig_average/2D_17_clone_h_no_cut_mmdt_FastJets04MultLam100__herwig_average.pdf} 
        %%for now \includegraphics[width=8cm]{./figures/angs2D_filter_herwig_average/2D_5_clone_h_no_cut_mmdt_FastJets10MultLam100__herwig_average.pdf} 
        %%for now \caption{2D Multiplicity $R=0.4$ (left), $R=1.0$ (right).}
        \end{figure}
        
        %%% Lha %%%
        \begin{figure}[h!]
        \centering
        \includegraphics[width=8cm]{./figures/angs1D_filter_herwig_average/1D_X20Y15Z140W11T73R8_clone_h_no_cut_mmdt_FastJets04LhaLam100__herwig_average.pdf} 
        \includegraphics[width=8cm]{./figures/angs1D_filter_herwig_average/1D_X10Y115Z452W14T12R3_clone_h_no_cut_mmdt_FastJets10LhaLam100__herwig_average.pdf} 
        \caption{Quark and Gluon averaged angularities $\lambda_{0.5}^{1}$ - left R = 0.4, right R = 1.0. 
        Using \herwig{} event generator, at Q100 region, using average of 6 energy combinations 
        900-2360, 900-7000, 900-13000, 2360-7000, 2360-13000, 7000-13000~GeV.}
        \label{fig:mmdt_lha2}
    
        %%for now \includegraphics[width=8cm]{./figures/angs2D_filter_herwig_average/2D_13_clone_h_no_cut_mmdt_FastJets04LhaLam100__herwig_average.pdf} 
        %%for now \includegraphics[width=8cm]{./figures/angs2D_filter_herwig_average/2D_5_clone_h_no_cut_mmdt_FastJets10LhaLam100__herwig_average.pdf} 
        %%for now \caption{2D Lha $R=0.4$ (left), $R=1.0$ (right).}
        \end{figure}
        
        %%% Width %%%
        \begin{figure}[h!]
        \centering
        \includegraphics[width=8cm]{./figures/angs1D_filter_herwig_average/1D_X17Y12Z136W10T81R7_clone_h_no_cut_mmdt_FastJets04WidthLam100__herwig_average.pdf} 
        \includegraphics[width=8cm]{./figures/angs1D_filter_herwig_average/1D_X9Y117Z684W13T11R2_clone_h_no_cut_mmdt_FastJets10WidthLam100__herwig_average.pdf} 
        \caption{Quark and Gluon averaged angularities $\lambda_{1}^{1}$ - left R = 0.4, right R = 1.0. 
        Using \herwig{} event generator, at Q100 region, using average of 6 energy combinations 
        900-2360, 900-7000, 900-13000, 2360-7000, 2360-13000, 7000-13000~GeV.}
        \label{fig:mmdt_width2}
    
        %%for now \includegraphics[width=8cm]{./figures/angs2D_filter_herwig_average/2D_X11Y-nanZ43_clone_h_no_cut_mmdt_FastJets04WidthLam100__herwig_average.pdf} 
        %%for now \includegraphics[width=8cm]{./figures/angs2D_filter_herwig_average/2D_4_clone_h_no_cut_mmdt_FastJets10WidthLam100__herwig_average.pdf} 
        %%for now \caption{2D Width $R=0.4$ (left), $R=1.0$ (right).}
        \end{figure}
        
        %%% Pt %%%
        \begin{figure}[h!]
        \centering
        \includegraphics[width=8cm]{./figures/angs1D_filter_herwig_average/1D_X66Y12Z58W17T144R29_clone_h_no_cut_mmdt_FastJets04PtLam100__herwig_average.pdf} 
        \includegraphics[width=8cm]{./figures/angs1D_filter_herwig_average/1D_X12Y77Z210W21T27R10_clone_h_no_cut_mmdt_FastJets10PtLam100__herwig_average.pdf} 
        \caption{Quark and Gluon averaged angularities $\lambda_{0}^{2}$ - left R = 0.4, right R = 1.0. 
        Using \herwig{} event generator, at Q100 region, using average of 6 energy combinations 
        900-2360, 900-7000, 900-13000, 2360-7000, 2360-13000, 7000-13000~GeV.}
        \label{fig:mmdt_pt2}
        %%for now \includegraphics[width=8cm]{./figures/angs2D_filter_herwig_average/2D_42_clone_h_no_cut_mmdt_FastJets04PtLam100__herwig_average.pdf} 
        %%for now \includegraphics[width=8cm]{./figures/angs2D_filter_herwig_average/2D_11_clone_h_no_cut_mmdt_FastJets10PtLam100__herwig_average.pdf} 
        %%for now \caption{2D Pt $R=0.4$ (left), $R=1.0$ (right).}
        \end{figure}
        
        %%% Mass %%%
        \begin{figure}[h!]
        \centering
        \includegraphics[width=8cm]{./figures/angs1D_filter_herwig_average/1D_X14Y19Z94W8T40R8_clone_h_no_cut_mmdt_FastJets04MassLam100__herwig_average.pdf} 
        \includegraphics[width=8cm]{./figures/angs1D_filter_herwig_average/1D_X6Y99Z345W10T10R3_clone_h_no_cut_mmdt_FastJets10MassLam100__herwig_average.pdf} 
        \caption{Quark and Gluon averaged angularities $\lambda_{2}^{1}$ - left R = 0.4, right R = 1.0. 
        Using \herwig{} event generator, at Q100 region, using average of 6 energy combinations 
        900-2360, 900-7000, 900-13000, 2360-7000, 2360-13000, 7000-13000~GeV.}
        \label{fig:mmdt_mass2}
        %%for now \includegraphics[width=8cm]{./figures/angs2D_filter_herwig_average/2D_14_clone_h_no_cut_mmdt_FastJets04MassLam100__herwig_average.pdf} 
        %%for now \includegraphics[width=8cm]{./figures/angs2D_filter_herwig_average/2D_2_clone_h_no_cut_mmdt_FastJets10MassLam100__herwig_average.pdf} 
        %%for now \caption{2D Mass $R=0.4$ (left), $R=1.0$ (right).}
        \end{figure}
        \clearpage
    %%%%%%%%%%%%%%%%%%PYTHIA RESULTS %%%%%%%%%%%%%%%%%%%%%%%%%%%%%%%%%%
    \subsection{\pythia{} 1D Approach, Six Enerrgy Variations, Q100, Trimmed Jets}
    \begin{itemize}
        \item 5 - angularities $\lambda_0^0$, $\lambda_{0.5}^1$, $\lambda_1^1$, $\lambda_0^2$, $\lambda_2^1$ 
        \item 2 - quark/gluon
        \item 1 - using trimmed jets 
        \item 2 - jet radii $R = 0.4, 1.0$
        \item 1 - average of 6 energy combinations: 900-2360, 900-7000, 900-13000, 2360-7000, 2360-13000, 7000-13000~GeV
        \item 1 - event generators \pythia{}
        \item 1 - region - dijet average $p_{T}$ cut (Q100)
        \item 2 - MPI and ISR switched on/off
        \item 1 - gluon fraction $f(p_{T})$ 1D approach
    \end{itemize}

    %%% Multiplicity %%%
    \begin{figure}[h!]
        \centering
        \includegraphics[width=8cm]{./figures/angs1D_filter_herwig_average/1D_X14Y92Z431W20T22R5_clone_h_no_cut_mmdt_FastJets04MultLam100__pythia_average.pdf} 
        \includegraphics[width=8cm]{./figures/angs1D_filter_herwig_average/1D_X2Y991Z3223W26T3R1_clone_h_no_cut_mmdt_FastJets10MultLam100__pythia_average.pdf} 
        \caption{Quark and Gluon averaged angularities $\lambda_{0}^{0}$ - left R = 0.4, right R = 1.0. 
        Using \pythia{} event generator, at Q100 region, using average of 6 energy combinations 
        900-2360, 900-7000, 900-13000, 2360-7000, 2360-13000, 7000-13000~GeV.}
        \label{fig:mmdt_mult2_pyt}
        %%for now \includegraphics[width=8cm]{./figures/angs2D_filter_herwig_average/2D_17_clone_h_no_cut_mmdt_FastJets04MultLam100__pythia_average.pdf} 
        %%for now \includegraphics[width=8cm]{./figures/angs2D_filter_herwig_average/2D_5_clone_h_no_cut_mmdt_FastJets10MultLam100__pythia_average.pdf} 
        %%for now \caption{2D Multiplicity $R=0.4$ (left), $R=1.0$ (right).}
        \end{figure}
        
        %%% Lha %%%
        \begin{figure}[h!]
        \centering
        \includegraphics[width=8cm]{./figures/angs1D_filter_herwig_average/1D_X19Y32Z133W11T35R9_clone_h_no_cut_mmdt_FastJets04LhaLam100__pythia_average.pdf} 
        \includegraphics[width=8cm]{./figures/angs1D_filter_herwig_average/1D_X4Y584Z2857W18T3R1_clone_h_no_cut_mmdt_FastJets10LhaLam100__pythia_average.pdf} 
        \caption{Quark and Gluon averaged angularities $\lambda_{0.5}^{1}$ - left R = 0.4, right R = 1.0. 
        Using \pythia{} event generator, at Q100 region, using average of 6 energy combinations 
        900-2360, 900-7000, 900-13000, 2360-7000, 2360-13000, 7000-13000~GeV.}
        \label{fig:mmdt_lha2_pyt}
    
        %%for now \includegraphics[width=8cm]{./figures/angs2D_filter_herwig_average/2D_X13Y21Z102_clone_h_no_cut_mmdt_FastJets04LhaLam100__pythia_average.pdf} 
        %%for now \includegraphics[width=8cm]{./figures/angs2D_filter_herwig_average/2D_5_clone_h_no_cut_mmdt_FastJets10LhaLam100__pythia_average.pdf} 
        %%for now \caption{2D Lha $R=0.4$ (left), $R=1.0$ (right).}
        \end{figure}
        
        %%% Width %%%
        \begin{figure}[h!]
        \centering
        \includegraphics[width=8cm]{./figures/angs1D_filter_herwig_average/1D_X15Y40Z186W10T25R5_clone_h_no_cut_mmdt_FastJets04WidthLam100__pythia_average.pdf} 
        \includegraphics[width=8cm]{./figures/angs1D_filter_herwig_average/1D_X3Y630Z2371W17T3R1_clone_h_no_cut_mmdt_FastJets10WidthLam100__pythia_average.pdf} 
        \caption{Quark and Gluon averaged angularities $\lambda_{1}^{1}$ - left R = 0.4, right R = 1.0. 
        Using \pythia{} event generator, at Q100 region, using average of 6 energy combinations 
        900-2360, 900-7000, 900-13000, 2360-7000, 2360-13000, 7000-13000~GeV.}
        \label{fig:mmdt_width2_pyt}
    
        %%for now \includegraphics[width=8cm]{./figures/angs2D_filter_herwig_average/2D_X12Y29Z146_clone_h_no_cut_mmdt_FastJets04WidthLam100__pythia_average.pdf} 
        %%for now \includegraphics[width=8cm]{./figures/angs2D_filter_herwig_average/2D_X4Y204Z952_clone_h_no_cut_mmdt_FastJets10WidthLam100__pythia_average.pdf} 
        %%for now \caption{2D Width $R=0.4$ (left), $R=1.0$ (right).}
        \end{figure}
        
        %%% Pt %%%
        \begin{figure}[h!]
        \centering
        \includegraphics[width=8cm]{./figures/angs1D_filter_herwig_average/1D_X31Y27Z164W18T66R11_clone_h_no_cut_mmdt_FastJets04PtLam100__pythia_average.pdf} 
        \includegraphics[width=8cm]{./figures/angs1D_filter_herwig_average/1D_X6Y217Z637W24T11R4_clone_h_no_cut_mmdt_FastJets10PtLam100__pythia_average.pdf} 
        \caption{Quark and Gluon averaged angularities $\lambda_{0}^{2}$ - left R = 0.4, right R = 1.0. 
        Using \pythia{} event generator, at Q100 region, using average of 6 energy combinations 
        900-2360, 900-7000, 900-13000, 2360-7000, 2360-13000, 7000-13000~GeV.}
        \label{fig:mmdt_pt2_pyt}
        %%for now \includegraphics[width=8cm]{./figures/angs2D_filter_herwig_average/2D_42_clone_h_no_cut_mmdt_FastJets04PtLam100__pythia_average.pdf} 
        %%for now \includegraphics[width=8cm]{./figures/angs2D_filter_herwig_average/2D_11_clone_h_no_cut_mmdt_FastJets10PtLam100__pythia_average.pdf} 
        %%for now \caption{2D Pt $R=0.4$ (left), $R=1.0$ (right).}
        \end{figure}
        
        %%% Mass %%%
        \begin{figure}[h!]
        \centering
        \includegraphics[width=8cm]{./figures/angs1D_filter_herwig_average/1D_X14Y40Z262W7T19R3_clone_h_no_cut_mmdt_FastJets04MassLam100__pythia_average.pdf} 
        \includegraphics[width=8cm]{./figures/angs1D_filter_herwig_average/1D_X2Y484Z2105W13T3R1_clone_h_no_cut_mmdt_FastJets10MassLam100__pythia_average.pdf} 
        \caption{Quark and Gluon averaged angularities $\lambda_{2}^{1}$ - left R = 0.4, right R = 1.0. 
        Using \pythia{} event generator, at Q100 region, using average of 6 energy combinations 
        900-2360, 900-7000, 900-13000, 2360-7000, 2360-13000, 7000-13000~GeV.}
        \label{fig:mmdt_mass2_pyt}
        %%for now \includegraphics[width=8cm]{./figures/angs2D_filter_herwig_average/2D_7_clone_h_no_cut_mmdt_FastJets04MassLam100__pythia_average.pdf} 
        %%for now \includegraphics[width=8cm]{./figures/angs2D_filter_herwig_average/2D_X3Y170Z983_clone_h_no_cut_mmdt_FastJets10MassLam100__pythia_average.pdf} 
        %%for now \caption{2D Mass $R=0.4$ (left), $R=1.0$ (right).}
        \end{figure}
        \clearpage
    %%%% 2D APPROACH%%%%%%%%%%%%%%%%%%%%%%%%%%%
    \subsection{\herwig{} 2D Approach, Six Enerrgy Variations, Q100, Trimmed Jets}
    \begin{itemize}
        \item 5 - angularities $\lambda_0^0$, $\lambda_{0.5}^1$, $\lambda_1^1$, $\lambda_0^2$, $\lambda_2^1$ 
        \item 2 - quark/gluon
        \item 1 - using trimmed jets 
        \item 2 - jet radii $R = 0.4, 1.0$
        \item 1 - average of 6 energy combinations: 900-2360, 900-7000, 900-13000, 2360-7000, 2360-13000, 7000-13000~GeV
        \item 1 - event generators \herwig{}
        \item 1 - region - dijet average $p_{T}$ cut (Q100)
        \item 2 - MPI and ISR switched on/off
        \item 1 - gluon fraction $f(p_{T})$ 2D approach
    \end{itemize}

    %%% Multiplicity %%%
    \begin{figure}[h!]
        \centering
        \includegraphics[width=8cm]{./figures/angs2D_filter_herwig_average/2D_X28Y20Z42_clone_h_no_cut_mmdt_FastJets04MultLam100__herwig_average.pdf} 
        \includegraphics[width=8cm]{./figures/angs2D_filter_herwig_average/2D_X9Y69Z175_clone_h_no_cut_mmdt_FastJets10MultLam100__herwig_average.pdf} 
        \caption{Quark and Gluon averaged angularities $\lambda_{0}^{0}$ - left R = 0.4, right R = 1.0. 
        Using \herwig{} event generator, at Q100 region, using average of 6 energy combinations 
        900-2360, 900-7000, 900-13000, 2360-7000, 2360-13000, 7000-13000~GeV.}
        \label{fig:mmdt_2D_mult2}
        %%for now \includegraphics[width=8cm]{./figures/angs2D_filter_herwig_average/2D_17_clone_h_no_cut_mmdt_FastJets04MultLam100__herwig_average.pdf} 
        %%for now \includegraphics[width=8cm]{./figures/angs2D_filter_herwig_average/2D_5_clone_h_no_cut_mmdt_FastJets10MultLam100__herwig_average.pdf} 
        %%for now \caption{2D Multiplicity $R=0.4$ (left), $R=1.0$ (right).}
        \end{figure}
        
        %%% Lha %%%
        \begin{figure}[h!]
        \centering
        \includegraphics[width=8cm]{./figures/angs2D_filter_herwig_average/2D_X12Y11Z55_clone_h_no_cut_mmdt_FastJets04LhaLam100__herwig_average.pdf} 
        \includegraphics[width=8cm]{./figures/angs2D_filter_herwig_average/2D_X10Y48Z213_clone_h_no_cut_mmdt_FastJets10LhaLam100__herwig_average.pdf} 
        \caption{Quark and Gluon averaged angularities $\lambda_{0.5}^{1}$ - left R = 0.4, right R = 1.0. 
        Using \herwig{} event generator, at Q100 region, using average of 6 energy combinations 
        900-2360, 900-7000, 900-13000, 2360-7000, 2360-13000, 7000-13000~GeV.}
        \label{fig:mmdt_2D_lha2}
    
        %%for now \includegraphics[width=8cm]{./figures/angs2D_filter_herwig_average/2D_13_clone_h_no_cut_mmdt_FastJets04LhaLam100__herwig_average.pdf} 
        %%for now \includegraphics[width=8cm]{./figures/angs2D_filter_herwig_average/2D_5_clone_h_no_cut_mmdt_FastJets10LhaLam100__herwig_average.pdf} 
        %%for now \caption{2D Lha $R=0.4$ (left), $R=1.0$ (right).}
        \end{figure}
        
        %%% Width %%%
        \begin{figure}[h!]
        \centering
        \includegraphics[width=8cm]{./figures/angs2D_filter_herwig_average/2D_X11Y-nanZ43_clone_h_no_cut_mmdt_FastJets04WidthLam100__herwig_average.pdf} 
        \includegraphics[width=8cm]{./figures/angs2D_filter_herwig_average/2D_X9Y52Z217_clone_h_no_cut_mmdt_FastJets10WidthLam100__herwig_average.pdf} 
        \caption{Quark and Gluon averaged angularities $\lambda_{1}^{1}$ - left R = 0.4, right R = 1.0. 
        Using \herwig{} event generator, at Q100 region, using average of 6 energy combinations 
        900-2360, 900-7000, 900-13000, 2360-7000, 2360-13000, 7000-13000~GeV.}
        \label{fig:mmdt_2D_width2}
    
        %%for now \includegraphics[width=8cm]{./figures/angs2D_filter_herwig_average/2D_X11Y-nanZ43_clone_h_no_cut_mmdt_FastJets04WidthLam100__herwig_average.pdf} 
        %%for now \includegraphics[width=8cm]{./figures/angs2D_filter_herwig_average/2D_4_clone_h_no_cut_mmdt_FastJets10WidthLam100__herwig_average.pdf} 
        %%for now \caption{2D Width $R=0.4$ (left), $R=1.0$ (right).}
        \end{figure}
        
        %%% Pt %%%
        \begin{figure}[h!]
        \centering
        \includegraphics[width=8cm]{./figures/angs2D_filter_herwig_average/2D_X61Y6Z20_clone_h_no_cut_mmdt_FastJets04PtLam100__herwig_average.pdf} 
        \includegraphics[width=8cm]{./figures/angs2D_filter_herwig_average/2D_X17Y30Z69_clone_h_no_cut_mmdt_FastJets10PtLam100__herwig_average.pdf} 
        \caption{Quark and Gluon averaged angularities $\lambda_{0}^{2}$ - left R = 0.4, right R = 1.0. 
        Using \herwig{} event generator, at Q100 region, using average of 6 energy combinations 
        900-2360, 900-7000, 900-13000, 2360-7000, 2360-13000, 7000-13000~GeV.}
        \label{fig:mmdt_2D_pt2}
        %%for now \includegraphics[width=8cm]{./figures/angs2D_filter_herwig_average/2D_42_clone_h_no_cut_mmdt_FastJets04PtLam100__herwig_average.pdf} 
        %%for now \includegraphics[width=8cm]{./figures/angs2D_filter_herwig_average/2D_11_clone_h_no_cut_mmdt_FastJets10PtLam100__herwig_average.pdf} 
        %%for now \caption{2D Pt $R=0.4$ (left), $R=1.0$ (right).}
        \end{figure}
        
        %%% Mass %%%
        \begin{figure}[h!]
        \centering
        \includegraphics[width=8cm]{./figures/angs2D_filter_herwig_average/2D_X11Y11Z70_clone_h_no_cut_mmdt_FastJets04MassLam100__herwig_average.pdf} 
        \includegraphics[width=8cm]{./figures/angs2D_filter_herwig_average/2D_X7Y39Z174_clone_h_no_cut_mmdt_FastJets10MassLam100__herwig_average.pdf} 
        \caption{Quark and Gluon averaged angularities $\lambda_{2}^{1}$ - left R = 0.4, right R = 1.0. 
        Using \herwig{} event generator, at Q100 region, using average of 6 energy combinations 
        900-2360, 900-7000, 900-13000, 2360-7000, 2360-13000, 7000-13000~GeV.}
        \label{fig:mmdt_2D_mass2}
        %%for now \includegraphics[width=8cm]{./figures/angs2D_filter_herwig_average/2D_7_clone_h_no_cut_mmdt_FastJets04MassLam100__herwig_average.pdf} 
        %%for now \includegraphics[width=8cm]{./figures/angs2D_filter_herwig_average/2D_3_clone_h_no_cut_mmdt_FastJets10MassLam100__herwig_average.pdf} 
        %%for now \caption{2D Mass $R=0.4$ (left), $R=1.0$ (right).}
        \end{figure}
        \clearpage
    %%%%%%%%%%%%%%%%%%PYTHIA RESULTS %%%%%%%%%%%%%%%%%%%%%%%%%%%%%%%%%%
    \subsection{\pythia{} 2D Approach, Six Enerrgy Variations, Q100, Trimmed Jets}
    \begin{itemize}
        \item 5 - angularities $\lambda_0^0$, $\lambda_{0.5}^1$, $\lambda_1^1$, $\lambda_0^2$, $\lambda_2^1$ 
        \item 2 - quark/gluon
        \item 1 - using trimmed jets 
        \item 2 - jet radii $R = 0.4, 1.0$
        \item 1 - average of 6 energy combinations: 900-2360, 900-7000, 900-13000, 2360-7000, 2360-13000, 7000-13000~GeV
        \item 1 - event generators \pythia{}
        \item 1 - region - dijet average $p_{T}$ cut (Q100)
        \item 2 - MPI and ISR switched on/off
        \item 1 - gluon fraction $f(p_{T})$ 2D approach
    \end{itemize}

    %%% Multiplicity %%%
    \begin{figure}[h!]
        \centering
        \includegraphics[width=8cm]{./figures/angs2D_filter_herwig_average/2D_X15Y47Z140_clone_h_no_cut_mmdt_FastJets04MultLam100__pythia_average.pdf} 
        \includegraphics[width=8cm]{./figures/angs2D_filter_herwig_average/2D_X2Y361Z790_clone_h_no_cut_mmdt_FastJets10MultLam100__pythia_average.pdf} 
        \caption{Quark and Gluon averaged angularities $\lambda_{0}^{0}$ - left R = 0.4, right R = 1.0. 
        Using \pythia{} event generator, at Q100 region, using average of 6 energy combinations 
        900-2360, 900-7000, 900-13000, 2360-7000, 2360-13000, 7000-13000~GeV.}
        \label{fig:mmdt_2D_mult2_pyt}
        %%for now \includegraphics[width=8cm]{./figures/angs2D_filter_herwig_average/2D_17_clone_h_no_cut_mmdt_FastJets04MultLam100__pythia_average.pdf} 
        %%for now \includegraphics[width=8cm]{./figures/angs2D_filter_herwig_average/2D_5_clone_h_no_cut_mmdt_FastJets10MultLam100__pythia_average.pdf} 
        %%for now \caption{2D Multiplicity $R=0.4$ (left), $R=1.0$ (right).}
        \end{figure}
        
        %%% Lha %%%
        \begin{figure}[h!]
        \centering
        \includegraphics[width=8cm]{./figures/angs2D_filter_herwig_average/2D_X13Y21Z102_clone_h_no_cut_mmdt_FastJets04LhaLam100__pythia_average.pdf} 
        \includegraphics[width=8cm]{./figures/angs2D_filter_herwig_average/2D_X4Y202Z839_clone_h_no_cut_mmdt_FastJets10LhaLam100__pythia_average.pdf} 
        \caption{Quark and Gluon averaged angularities $\lambda_{0.5}^{1}$ - left R = 0.4, right R = 1.0. 
        Using \pythia{} event generator, at Q100 region, using average of 6 energy combinations 
        900-2360, 900-7000, 900-13000, 2360-7000, 2360-13000, 7000-13000~GeV.}
        \label{fig:mmdt_2D_lha2_pyt}
    
        %%for now \includegraphics[width=8cm]{./figures/angs2D_filter_herwig_average/2D_X13Y21Z102_clone_h_no_cut_mmdt_FastJets04LhaLam100__pythia_average.pdf} 
        %%for now \includegraphics[width=8cm]{./figures/angs2D_filter_herwig_average/2D_5_clone_h_no_cut_mmdt_FastJets10LhaLam100__pythia_average.pdf} 
        %%for now \caption{2D Lha $R=0.4$ (left), $R=1.0$ (right).}
        \end{figure}
        
        %%% Width %%%
        \begin{figure}[h!]
        \centering
        \includegraphics[width=8cm]{./figures/angs2D_filter_herwig_average/2D_X12Y29Z146_clone_h_no_cut_mmdt_FastJets04WidthLam100__pythia_average.pdf} 
        \includegraphics[width=8cm]{./figures/angs2D_filter_herwig_average/2D_X4Y204Z952_clone_h_no_cut_mmdt_FastJets10WidthLam100__pythia_average.pdf} 
        \caption{Quark and Gluon averaged angularities $\lambda_{1}^{1}$ - left R = 0.4, right R = 1.0. 
        Using \pythia{} event generator, at Q100 region, using average of 6 energy combinations 
        900-2360, 900-7000, 900-13000, 2360-7000, 2360-13000, 7000-13000~GeV.}
        \label{fig:mmdt_2D_width2_pyt}
    
        %%for now \includegraphics[width=8cm]{./figures/angs2D_filter_herwig_average/2D_X12Y29Z146_clone_h_no_cut_mmdt_FastJets04WidthLam100__pythia_average.pdf} 
        %%for now \includegraphics[width=8cm]{./figures/angs2D_filter_herwig_average/2D_X4Y204Z952_clone_h_no_cut_mmdt_FastJets10WidthLam100__pythia_average.pdf} 
        %%for now \caption{2D Width $R=0.4$ (left), $R=1.0$ (right).}
        \end{figure}
        
        %%% Pt %%%
        \begin{figure}[h!]
        \centering
        \includegraphics[width=8cm]{./figures/angs2D_filter_herwig_average/2D_X27Y17Z72_clone_h_no_cut_mmdt_FastJets04PtLam100__pythia_average.pdf} 
        \includegraphics[width=8cm]{./figures/angs2D_filter_herwig_average/2D_X7Y73Z207_clone_h_no_cut_mmdt_FastJets10PtLam100__pythia_average.pdf} 
        \caption{Quark and Gluon averaged angularities $\lambda_{0}^{2}$ - left R = 0.4, right R = 1.0. 
        Using \pythia{} event generator, at Q100 region, using average of 6 energy combinations 
        900-2360, 900-7000, 900-13000, 2360-7000, 2360-13000, 7000-13000~GeV.}
        \label{fig:mmdt_2D_pt2_pyt}
        %%for now \includegraphics[width=8cm]{./figures/angs2D_filter_herwig_average/2D_42_clone_h_no_cut_mmdt_FastJets04PtLam100__pythia_average.pdf} 
        %%for now \includegraphics[width=8cm]{./figures/angs2D_filter_herwig_average/2D_11_clone_h_no_cut_mmdt_FastJets10PtLam100__pythia_average.pdf} 
        %%for now \caption{2D Pt $R=0.4$ (left), $R=1.0$ (right).}
        \end{figure}
        
        %%% Mass %%%
        \begin{figure}[h!]
        \centering
        \includegraphics[width=8cm]{./figures/angs2D_filter_herwig_average/2D_X13Y18Z165_clone_h_no_cut_mmdt_FastJets04MassLam100__pythia_average.pdf} 
        \includegraphics[width=8cm]{./figures/angs2D_filter_herwig_average/2D_X3Y170Z983_clone_h_no_cut_mmdt_FastJets10MassLam100__pythia_average.pdf} 
        \caption{Quark and Gluon averaged angularities $\lambda_{2}^{1}$ - left R = 0.4, right R = 1.0. 
        Using \pythia{} event generator, at Q100 region, using average of 6 energy combinations 
        900-2360, 900-7000, 900-13000, 2360-7000, 2360-13000, 7000-13000~GeV.}
        \label{fig:mmdt_2D_mass2_pyt}
        %%for now \includegraphics[width=8cm]{./figures/angs2D_filter_herwig_average/2D_7_clone_h_no_cut_mmdt_FastJets04MassLam100__pythia_average.pdf} 
        %%for now \includegraphics[width=8cm]{./figures/angs2D_filter_herwig_average/2D_X3Y170Z983_clone_h_no_cut_mmdt_FastJets10MassLam100__pythia_average.pdf} 
        %%for now \caption{2D Mass $R=0.4$ (left), $R=1.0$ (right).}
        \end{figure}
        \clearpage
    
%%%%%%%%%%%%Q50 results 

\subsection{\herwig{} 1D Approach, Six Enerrgy Variations, Q50}
\begin{itemize}
    \item 5 - angularities $\lambda_0^0$, $\lambda_{0.5}^1$, $\lambda_1^1$, $\lambda_0^2$, $\lambda_2^1$ 
    \item 2 - quark/gluon
    \item 1 - using no trimmed jets 
    \item 2 - jet radii $R = 0.4, 1.0$
    \item 1 - average of 6 energy combinations: 900-2360, 900-7000, 900-13000, 2360-7000, 2360-13000, 7000-13000~GeV
    \item 1 - event generators \herwig{}
    \item 1 - region - dijet average $p_{T}$ cut (Q50)
    \item 2 - MPI and ISR switched on/off
    \item 1 - gluon fraction $f(p_{T})$ 1D approach
\end{itemize}

%%% Multiplicity %%%
\begin{figure}[h!]
    \centering
    \includegraphics[width=8cm]{./figures/angs1D_filter_herwig_average/1D_X16Y26Z68W60T230R88_clone_h_no_cut_FastJets04MultLam50__herwig_average.pdf} 
    \includegraphics[width=8cm]{./figures/angs1D_filter_herwig_average/1D_X4Y34Z279W83T241R30_clone_h_no_cut_FastJets10MultLam50__herwig_average.pdf} 
    \caption{Quark and Gluon averaged angularities $\lambda_{0}^{0}$ - left R = 0.4, right R = 1.0. 
    Using \herwig{} event generator, at Q50 region, using average of 6 energy combinations 
    900-2360, 900-7000, 900-13000, 2360-7000, 2360-13000, 7000-13000~GeV.}
    \label{fig:Q50_mult2}
    %%for now \includegraphics[width=8cm]{./figures/angs2D_filter_herwig_average/2D_17_clone_h_no_cut_FastJets04MultLam50__herwig_average.pdf} 
    %%for now \includegraphics[width=8cm]{./figures/angs2D_filter_herwig_average/2D_5_clone_h_no_cut_FastJets10MultLam50__herwig_average.pdf} 
    %%for now \caption{2D Multiplicity $R=0.4$ (left), $R=1.0$ (right).}
    \end{figure}
    
    %%% Lha %%%
    \begin{figure}[h!]
    \centering
    \includegraphics[width=8cm]{./figures/angs1D_filter_herwig_average/1D_X5Y20Z124W38T193R31_clone_h_no_cut_FastJets04LhaLam50__herwig_average.pdf} 
    \includegraphics[width=8cm]{./figures/angs1D_filter_herwig_average/1D_X2Y153Z240W73T48R30_clone_h_no_cut_FastJets10LhaLam50__herwig_average.pdf} 
    \caption{Quark and Gluon averaged angularities $\lambda_{0.5}^{1}$ - left R = 0.4, right R = 1.0. 
    Using \herwig{} event generator, at Q50 region, using average of 6 energy combinations 
    900-2360, 900-7000, 900-13000, 2360-7000, 2360-13000, 7000-13000~GeV.}
    \label{fig:Q50_lha2}

    %%for now \includegraphics[width=8cm]{./figures/angs2D_filter_herwig_average/2D_13_clone_h_no_cut_FastJets04LhaLam50__herwig_average.pdf} 
    %%for now \includegraphics[width=8cm]{./figures/angs2D_filter_herwig_average/2D_5_clone_h_no_cut_FastJets10LhaLam50__herwig_average.pdf} 
    %%for now \caption{2D Lha $R=0.4$ (left), $R=1.0$ (right).}
    \end{figure}
    
    %%% Width %%%
    \begin{figure}[h!]
    \centering
    \includegraphics[width=8cm]{./figures/angs1D_filter_herwig_average/1D_X4Y30Z122W40T133R32_clone_h_no_cut_FastJets04WidthLam50__herwig_average.pdf} 
    \includegraphics[width=8cm]{./figures/angs1D_filter_herwig_average/1D_X2Y156Z225W75T48R33_clone_h_no_cut_FastJets10WidthLam50__herwig_average.pdf} 
    \caption{Quark and Gluon averaged angularities $\lambda_{1}^{1}$ - left R = 0.4, right R = 1.0. 
    Using \herwig{} event generator, at Q50 region, using average of 6 energy combinations 
    900-2360, 900-7000, 900-13000, 2360-7000, 2360-13000, 7000-13000~GeV.}
    \label{fig:Q50_width2}

    %%for now \includegraphics[width=8cm]{./figures/angs2D_filter_herwig_average/2D_11_clone_h_no_cut_FastJets04WidthLam50__herwig_average.pdf} 
    %%for now \includegraphics[width=8cm]{./figures/angs2D_filter_herwig_average/2D_4_clone_h_no_cut_FastJets10WidthLam50__herwig_average.pdf} 
    %%for now \caption{2D Width $R=0.4$ (left), $R=1.0$ (right).}
    \end{figure}
    
    %%% Pt %%%
    \begin{figure}[h!]
    \centering
    \includegraphics[width=8cm]{./figures/angs1D_filter_herwig_average/1D_X20Y15Z106W41T271R38_clone_h_no_cut_FastJets04PtLam50__herwig_average.pdf} 
    \includegraphics[width=8cm]{./figures/angs1D_filter_herwig_average/1D_X3Y71Z99W63T88R63_clone_h_no_cut_FastJets10PtLam50__herwig_average.pdf} 
    \caption{Quark and Gluon averaged angularities $\lambda_{0}^{2}$ - left R = 0.4, right R = 1.0. 
    Using \herwig{} event generator, at Q50 region, using average of 6 energy combinations 
    900-2360, 900-7000, 900-13000, 2360-7000, 2360-13000, 7000-13000~GeV.}
    \label{fig:Q50_pt2}
    %%for now \includegraphics[width=8cm]{./figures/angs2D_filter_herwig_average/2D_42_clone_h_no_cut_FastJets04PtLam50__herwig_average.pdf} 
    %%for now \includegraphics[width=8cm]{./figures/angs2D_filter_herwig_average/2D_11_clone_h_no_cut_FastJets10PtLam50__herwig_average.pdf} 
    %%for now \caption{2D Pt $R=0.4$ (left), $R=1.0$ (right).}
    \end{figure}
    
    %%% Mass %%%
    \begin{figure}[h!]
    \centering
    \includegraphics[width=8cm]{./figures/angs1D_filter_herwig_average/1D_X3Y32Z158W40T127R26_clone_h_no_cut_FastJets04MassLam50__herwig_average.pdf} 
    \includegraphics[width=8cm]{./figures/angs1D_filter_herwig_average/1D_X2Y167Z337W78T47R23_clone_h_no_cut_FastJets10MassLam50__herwig_average.pdf} 
    \caption{Quark and Gluon averaged angularities $\lambda_{2}^{1}$ - left R = 0.4, right R = 1.0. 
    Using \herwig{} event generator, at Q50 region, using average of 6 energy combinations 
    900-2360, 900-7000, 900-13000, 2360-7000, 2360-13000, 7000-13000~GeV.}
    \label{fig:Q50_mass2}
    %%for now \includegraphics[width=8cm]{./figures/angs2D_filter_herwig_average/2D_7_clone_h_no_cut_FastJets04MassLam50__herwig_average.pdf} 
    %%for now \includegraphics[width=8cm]{./figures/angs2D_filter_herwig_average/2D_3_clone_h_no_cut_FastJets10MassLam50__herwig_average.pdf} 
    %%for now \caption{2D Mass $R=0.4$ (left), $R=1.0$ (right).}
    \end{figure}
    \clearpage
%%%%%%%%%%%%%%%%%%PYTHIA RESULTS %%%%%%%%%%%%%%%%%%%%%%%%%%%%%%%%%%
\subsection{\pythia{} 1D Approach, Six Enerrgy Variations, Q50}
\begin{itemize}
    \item 5 - angularities $\lambda_0^0$, $\lambda_{0.5}^1$, $\lambda_1^1$, $\lambda_0^2$, $\lambda_2^1$ 
    \item 2 - quark/gluon
    \item 1 - using no trimmed jets 
    \item 2 - jet radii $R = 0.4, 1.0$
    \item 1 - average of 6 energy combinations: 900-2360, 900-7000, 900-13000, 2360-7000, 2360-13000, 7000-13000~GeV
    \item 1 - event generators \pythia{}
    \item 1 - region - dijet average $p_{T}$ cut (Q50)
    \item 2 - MPI and ISR switched on/off
    \item 1 - gluon fraction $f(p_{T})$ 1D approach
\end{itemize}

%%% Multiplicity %%%
\begin{figure}[h!]
    \centering
    \includegraphics[width=8cm]{./figures/angs1D_filter_herwig_average/1D_X4Y130Z261W65T50R25_clone_h_no_cut_FastJets04MultLam50__pythia_average.pdf} 
    \includegraphics[width=8cm]{./figures/angs1D_filter_herwig_average/1D_X1Y-nanZ1753W85T-nanR5_clone_h_no_cut_FastJets10MultLam50__pythia_average.pdf} 
    \caption{Quark and Gluon averaged angularities $\lambda_{0}^{0}$ - left R = 0.4, right R = 1.0. 
    Using \pythia{} event generator, at Q50 region, using average of 6 energy combinations 
    900-2360, 900-7000, 900-13000, 2360-7000, 2360-13000, 7000-13000~GeV.}
    \label{fig:Q50_mult2_pyt}
    %%for now \includegraphics[width=8cm]{./figures/angs2D_filter_herwig_average/2D_17_clone_h_no_cut_FastJets04MultLam50__pythia_average.pdf} 
    %%for now \includegraphics[width=8cm]{./figures/angs2D_filter_herwig_average/2D_5_clone_h_no_cut_FastJets10MultLam50__pythia_average.pdf} 
    %%for now \caption{2D Multiplicity $R=0.4$ (left), $R=1.0$ (right).}
    \end{figure}
    
    %%% Lha %%%
    \begin{figure}[h!]
    \centering
    \includegraphics[width=8cm]{./figures/angs1D_filter_herwig_average/1D_X6Y50Z257W39T80R15_clone_h_no_cut_FastJets04LhaLam50__pythia_average.pdf} 
    \includegraphics[width=8cm]{./figures/angs1D_filter_herwig_average/1D_X1Y318Z485W77T24R16_clone_h_no_cut_FastJets10LhaLam50__pythia_average.pdf} 
    \caption{Quark and Gluon averaged angularities $\lambda_{0.5}^{1}$ - left R = 0.4, right R = 1.0. 
    Using \pythia{} event generator, at Q50 region, using average of 6 energy combinations 
    900-2360, 900-7000, 900-13000, 2360-7000, 2360-13000, 7000-13000~GeV.}
    \label{fig:Q50_lha2_pyt}

    %%for now \includegraphics[width=8cm]{./figures/angs2D_filter_herwig_average/2D_13_clone_h_no_cut_FastJets04LhaLam50__pythia_average.pdf} 
    %%for now \includegraphics[width=8cm]{./figures/angs2D_filter_herwig_average/2D_5_clone_h_no_cut_FastJets10LhaLam50__pythia_average.pdf} 
    %%for now \caption{2D Lha $R=0.4$ (left), $R=1.0$ (right).}
    \end{figure}
    
    %%% Width %%%
    \begin{figure}[h!]
    \centering
    \includegraphics[width=8cm]{./figures/angs1D_filter_herwig_average/1D_X5Y53Z298W40T76R13_clone_h_no_cut_FastJets04WidthLam50__pythia_average.pdf} 
    \includegraphics[width=8cm]{./figures/angs1D_filter_herwig_average/1D_X1Y425Z593W81T19R14_clone_h_no_cut_FastJets10WidthLam50__pythia_average.pdf} 
    \caption{Quark and Gluon averaged angularities $\lambda_{1}^{1}$ - left R = 0.4, right R = 1.0. 
    Using \pythia{} event generator, at Q50 region, using average of 6 energy combinations 
    900-2360, 900-7000, 900-13000, 2360-7000, 2360-13000, 7000-13000~GeV.}
    \label{fig:Q50_width2_pyt}

    %%for now \includegraphics[width=8cm]{./figures/angs2D_filter_herwig_average/2D_11_clone_h_no_cut_FastJets04WidthLam50__pythia_average.pdf} 
    %%for now \includegraphics[width=8cm]{./figures/angs2D_filter_herwig_average/2D_4_clone_h_no_cut_FastJets10WidthLam50__pythia_average.pdf} 
    %%for now \caption{2D Width $R=0.4$ (left), $R=1.0$ (right).}
    \end{figure}
    
    %%% Pt %%%
    \begin{figure}[h!]
    \centering
    \includegraphics[width=8cm]{./figures/angs1D_filter_herwig_average/1D_X14Y22Z120W45T202R37_clone_h_no_cut_FastJets04PtLam50__pythia_average.pdf} 
    \includegraphics[width=8cm]{./figures/angs1D_filter_herwig_average/1D_X1Y149Z203W69T47R34_clone_h_no_cut_FastJets10PtLam50__pythia_average.pdf} 
    \caption{Quark and Gluon averaged angularities $\lambda_{0}^{2}$ - left R = 0.4, right R = 1.0. 
    Using \pythia{} event generator, at Q50 region, using average of 6 energy combinations 
    900-2360, 900-7000, 900-13000, 2360-7000, 2360-13000, 7000-13000~GeV.}
    \label{fig:Q50_pt2_pyt}
    %%for now \includegraphics[width=8cm]{./figures/angs2D_filter_herwig_average/2D_42_clone_h_no_cut_FastJets04PtLam50__pythia_average.pdf} 
    %%for now \includegraphics[width=8cm]{./figures/angs2D_filter_herwig_average/2D_11_clone_h_no_cut_FastJets10PtLam50__pythia_average.pdf} 
    %%for now \caption{2D Pt $R=0.4$ (left), $R=1.0$ (right).}
    \end{figure}
    
    %%% Mass %%%
    \begin{figure}[h!]
    \centering
    \includegraphics[width=8cm]{./figures/angs1D_filter_herwig_average/1D_X4Y55Z179W42T76R23_clone_h_no_cut_FastJets04MassLam50__pythia_average.pdf} 
    \includegraphics[width=8cm]{./figures/angs1D_filter_herwig_average/1D_X1Y541Z720W82T15R11_clone_h_no_cut_FastJets10MassLam50__pythia_average.pdf} 
    \caption{Quark and Gluon averaged angularities $\lambda_{2}^{1}$ - left R = 0.4, right R = 1.0. 
    Using \pythia{} event generator, at Q50 region, using average of 6 energy combinations 
    900-2360, 900-7000, 900-13000, 2360-7000, 2360-13000, 7000-13000~GeV.}
    \label{fig:Q50_mass2_pyt}
    %%for now \includegraphics[width=8cm]{./figures/angs2D_filter_herwig_average/2D_7_clone_h_no_cut_FastJets04MassLam50__pythia_average.pdf} 
    %%for now \includegraphics[width=8cm]{./figures/angs2D_filter_herwig_average/2D_3_clone_h_no_cut_FastJets10MassLam50__pythia_average.pdf} 
    %%for now \caption{2D Mass $R=0.4$ (left), $R=1.0$ (right).}
    \end{figure}
    \clearpage
%%%% 2D APPROACH%%%%%%%%%%%%%%%%%%%%%%%%%%%
\subsection{\herwig{} 2D Approach, Six Enerrgy Variations, Q50}
\begin{itemize}
    \item 5 - angularities $\lambda_0^0$, $\lambda_{0.5}^1$, $\lambda_1^1$, $\lambda_0^2$, $\lambda_2^1$ 
    \item 2 - quark/gluon
    \item 1 - using no trimmed jets 
    \item 2 - jet radii $R = 0.4, 1.0$
    \item 1 - average of 6 energy combinations: 900-2360, 900-7000, 900-13000, 2360-7000, 2360-13000, 7000-13000~GeV
    \item 1 - event generators \herwig{}
    \item 1 - region - dijet average $p_{T}$ cut (Q50)
    \item 2 - MPI and ISR switched on/off
    \item 1 - gluon fraction $f(p_{T})$ 2D approach
\end{itemize}

%%% Multiplicity %%%
\begin{figure}[h!]
    \centering
    \includegraphics[width=8cm]{./figures/angs2D_filter_herwig_average/2D_X12Y22Z80_clone_h_no_cut_FastJets04MultLam50__herwig_average.pdf} 
    \includegraphics[width=8cm]{./figures/angs2D_filter_herwig_average/2D_X4Y214Z457_clone_h_no_cut_FastJets10MultLam50__herwig_average.pdf} 
    \caption{Quark and Gluon averaged angularities $\lambda_{0}^{0}$ - left R = 0.4, right R = 1.0. 
    Using \herwig{} event generator, at Q50 region, using average of 6 energy combinations 
    900-2360, 900-7000, 900-13000, 2360-7000, 2360-13000, 7000-13000~GeV.}
    \label{fig:Q50_2D_mult2}
    %%for now \includegraphics[width=8cm]{./figures/angs2D_filter_herwig_average/2D_17_clone_h_no_cut_FastJets04MultLam50__herwig_average.pdf} 
    %%for now \includegraphics[width=8cm]{./figures/angs2D_filter_herwig_average/2D_5_clone_h_no_cut_FastJets10MultLam50__herwig_average.pdf} 
    %%for now \caption{2D Multiplicity $R=0.4$ (left), $R=1.0$ (right).}
    \end{figure}
    
    %%% Lha %%%
    \begin{figure}[h!]
    \centering
    \includegraphics[width=8cm]{./figures/angs2D_filter_herwig_average/2D_X5Y18Z97_clone_h_no_cut_FastJets04LhaLam50__herwig_average.pdf} 
    \includegraphics[width=8cm]{./figures/angs2D_filter_herwig_average/2D_X2Y137Z243_clone_h_no_cut_FastJets10LhaLam50__herwig_average.pdf} 
    \caption{Quark and Gluon averaged angularities $\lambda_{0.5}^{1}$ - left R = 0.4, right R = 1.0. 
    Using \herwig{} event generator, at Q50 region, using average of 6 energy combinations 
    900-2360, 900-7000, 900-13000, 2360-7000, 2360-13000, 7000-13000~GeV.}
    \label{fig:Q50_2D_lha2}

    %%for now \includegraphics[width=8cm]{./figures/angs2D_filter_herwig_average/2D_13_clone_h_no_cut_FastJets04LhaLam50__herwig_average.pdf} 
    %%for now \includegraphics[width=8cm]{./figures/angs2D_filter_herwig_average/2D_5_clone_h_no_cut_FastJets10LhaLam50__herwig_average.pdf} 
    %%for now \caption{2D Lha $R=0.4$ (left), $R=1.0$ (right).}
    \end{figure}
    
    %%% Width %%%
    \begin{figure}[h!]
    \centering
    \includegraphics[width=8cm]{./figures/angs2D_filter_herwig_average/2D_X4Y25Z122_clone_h_no_cut_FastJets04WidthLam50__herwig_average.pdf} 
    \includegraphics[width=8cm]{./figures/angs2D_filter_herwig_average/2D_X2Y143Z429_clone_h_no_cut_FastJets10WidthLam50__herwig_average.pdf} 
    \caption{Quark and Gluon averaged angularities $\lambda_{1}^{1}$ - left R = 0.4, right R = 1.0. 
    Using \herwig{} event generator, at Q50 region, using average of 6 energy combinations 
    900-2360, 900-7000, 900-13000, 2360-7000, 2360-13000, 7000-13000~GeV.}
    \label{fig:Q50_2D_width2}

    %%for now \includegraphics[width=8cm]{./figures/angs2D_filter_herwig_average/2D_11_clone_h_no_cut_FastJets04WidthLam50__herwig_average.pdf} 
    %%for now \includegraphics[width=8cm]{./figures/angs2D_filter_herwig_average/2D_4_clone_h_no_cut_FastJets10WidthLam50__herwig_average.pdf} 
    %%for now \caption{2D Width $R=0.4$ (left), $R=1.0$ (right).}
    \end{figure}
    
    %%% Pt %%%
    \begin{figure}[h!]
    \centering
    \includegraphics[width=8cm]{./figures/angs2D_filter_herwig_average/2D_X16Y12Z50_clone_h_no_cut_FastJets04PtLam50__herwig_average.pdf} 
    \includegraphics[width=8cm]{./figures/angs2D_filter_herwig_average/2D_X3Y55Z110_clone_h_no_cut_FastJets10PtLam50__herwig_average.pdf} 
    \caption{Quark and Gluon averaged angularities $\lambda_{0}^{2}$ - left R = 0.4, right R = 1.0. 
    Using \herwig{} event generator, at Q50 region, using average of 6 energy combinations 
    900-2360, 900-7000, 900-13000, 2360-7000, 2360-13000, 7000-13000~GeV.}
    \label{fig:Q50_2D_pt2}
    %%for now \includegraphics[width=8cm]{./figures/angs2D_filter_herwig_average/2D_42_clone_h_no_cut_FastJets04PtLam50__herwig_average.pdf} 
    %%for now \includegraphics[width=8cm]{./figures/angs2D_filter_herwig_average/2D_11_clone_h_no_cut_FastJets10PtLam50__herwig_average.pdf} 
    %%for now \caption{2D Pt $R=0.4$ (left), $R=1.0$ (right).}
    \end{figure}
    
    %%% Mass %%%
    \begin{figure}[h!]
    \centering
    \includegraphics[width=8cm]{./figures/angs2D_filter_herwig_average/2D_X4Y22Z112_clone_h_no_cut_FastJets04MassLam50__herwig_average.pdf} 
    \includegraphics[width=8cm]{./figures/angs2D_filter_herwig_average/2D_X2Y146Z265_clone_h_no_cut_FastJets10MassLam50__herwig_average.pdf} 
    \caption{Quark and Gluon averaged angularities $\lambda_{2}^{1}$ - left R = 0.4, right R = 1.0. 
    Using \herwig{} event generator, at Q50 region, using average of 6 energy combinations 
    900-2360, 900-7000, 900-13000, 2360-7000, 2360-13000, 7000-13000~GeV.}
    \label{fig:Q50_2D_mass2}
    %%for now \includegraphics[width=8cm]{./figures/angs2D_filter_herwig_average/2D_7_clone_h_no_cut_FastJets04MassLam50__herwig_average.pdf} 
    %%for now \includegraphics[width=8cm]{./figures/angs2D_filter_herwig_average/2D_3_clone_h_no_cut_FastJets10MassLam50__herwig_average.pdf} 
    %%for now \caption{2D Mass $R=0.4$ (left), $R=1.0$ (right).}
    \end{figure}
    \clearpage
%%%%%%%%%%%%%%%%%%PYTHIA RESULTS %%%%%%%%%%%%%%%%%%%%%%%%%%%%%%%%%%
\subsection{\pythia{} 2D Approach, Six Enerrgy Variations, Q50}
\begin{itemize}
    \item 5 - angularities $\lambda_0^0$, $\lambda_{0.5}^1$, $\lambda_1^1$, $\lambda_0^2$, $\lambda_2^1$ 
    \item 2 - quark/gluon
    \item 1 - using no trimmed jets 
    \item 2 - jet radii $R = 0.4, 1.0$
    \item 1 - average of 6 energy combinations: 900-2360, 900-7000, 900-13000, 2360-7000, 2360-13000, 7000-13000~GeV
    \item 1 - event generators \pythia{}
    \item 1 - region - dijet average $p_{T}$ cut (Q50)
    \item 2 - MPI and ISR switched on/off
    \item 1 - gluon fraction $f(p_{T})$ 2D approach
\end{itemize}

%%% Multiplicity %%%
\begin{figure}[h!]
    \centering
    \includegraphics[width=8cm]{./figures/angs2D_filter_herwig_average/2D_X4Y101Z181_clone_h_no_cut_FastJets04MultLam50__pythia_average.pdf} 
    \includegraphics[width=8cm]{./figures/angs2D_filter_herwig_average/2D_X1Y812Z2352_clone_h_no_cut_FastJets10MultLam50__pythia_average.pdf} 
    \caption{Quark and Gluon averaged angularities $\lambda_{0}^{0}$ - left R = 0.4, right R = 1.0. 
    Using \pythia{} event generator, at Q50 region, using average of 6 energy combinations 
    900-2360, 900-7000, 900-13000, 2360-7000, 2360-13000, 7000-13000~GeV.}
    \label{fig:Q50_2D_mult2_pyt}
    %%for now \includegraphics[width=8cm]{./figures/angs2D_filter_herwig_average/2D_17_clone_h_no_cut_FastJets04MultLam50__pythia_average.pdf} 
    %%for now \includegraphics[width=8cm]{./figures/angs2D_filter_herwig_average/2D_5_clone_h_no_cut_FastJets10MultLam50__pythia_average.pdf} 
    %%for now \caption{2D Multiplicity $R=0.4$ (left), $R=1.0$ (right).}
    \end{figure}
    
    %%% Lha %%%
    \begin{figure}[h!]
    \centering
    \includegraphics[width=8cm]{./figures/angs2D_filter_herwig_average/2D_X6Y45Z159_clone_h_no_cut_FastJets04LhaLam50__pythia_average.pdf} 
    \includegraphics[width=8cm]{./figures/angs2D_filter_herwig_average/2D_X1Y328Z687_clone_h_no_cut_FastJets10LhaLam50__pythia_average.pdf} 
    \caption{Quark and Gluon averaged angularities $\lambda_{0.5}^{1}$ - left R = 0.4, right R = 1.0. 
    Using \pythia{} event generator, at Q50 region, using average of 6 energy combinations 
    900-2360, 900-7000, 900-13000, 2360-7000, 2360-13000, 7000-13000~GeV.}
    \label{fig:Q50_2D_lha2_pyt}

    %%for now \includegraphics[width=8cm]{./figures/angs2D_filter_herwig_average/2D_13_clone_h_no_cut_FastJets04LhaLam50__pythia_average.pdf} 
    %%for now \includegraphics[width=8cm]{./figures/angs2D_filter_herwig_average/2D_5_clone_h_no_cut_FastJets10LhaLam50__pythia_average.pdf} 
    %%for now \caption{2D Lha $R=0.4$ (left), $R=1.0$ (right).}
    \end{figure}
    
    %%% Width %%%
    \begin{figure}[h!]
    \centering
    \includegraphics[width=8cm]{./figures/angs2D_filter_herwig_average/2D_X5Y50Z224_clone_h_no_cut_FastJets04WidthLam50__pythia_average.pdf} 
    \includegraphics[width=8cm]{./figures/angs2D_filter_herwig_average/2D_X1Y400Z630_clone_h_no_cut_FastJets10WidthLam50__pythia_average.pdf} 
    \caption{Quark and Gluon averaged angularities $\lambda_{1}^{1}$ - left R = 0.4, right R = 1.0. 
    Using \pythia{} event generator, at Q50 region, using average of 6 energy combinations 
    900-2360, 900-7000, 900-13000, 2360-7000, 2360-13000, 7000-13000~GeV.}
    \label{fig:Q50_2D_width2_pyt}

    %%for now \includegraphics[width=8cm]{./figures/angs2D_filter_herwig_average/2D_11_clone_h_no_cut_FastJets04WidthLam50__pythia_average.pdf} 
    %%for now \includegraphics[width=8cm]{./figures/angs2D_filter_herwig_average/2D_4_clone_h_no_cut_FastJets10WidthLam50__pythia_average.pdf} 
    %%for now \caption{2D Width $R=0.4$ (left), $R=1.0$ (right).}
    \end{figure}
    
    %%% Pt %%%
    \begin{figure}[h!]
    \centering
    \includegraphics[width=8cm]{./figures/angs2D_filter_herwig_average/2D_X11Y23Z112_clone_h_no_cut_FastJets04PtLam50__pythia_average.pdf} 
    \includegraphics[width=8cm]{./figures/angs2D_filter_herwig_average/2D_X1Y126Z328_clone_h_no_cut_FastJets10PtLam50__pythia_average.pdf} 
    \caption{Quark and Gluon averaged angularities $\lambda_{0}^{2}$ - left R = 0.4, right R = 1.0. 
    Using \pythia{} event generator, at Q50 region, using average of 6 energy combinations 
    900-2360, 900-7000, 900-13000, 2360-7000, 2360-13000, 7000-13000~GeV.}
    \label{fig:Q50_2D_pt2_pyt}
    %%for now \includegraphics[width=8cm]{./figures/angs2D_filter_herwig_average/2D_42_clone_h_no_cut_FastJets04PtLam50__pythia_average.pdf} 
    %%for now \includegraphics[width=8cm]{./figures/angs2D_filter_herwig_average/2D_11_clone_h_no_cut_FastJets10PtLam50__pythia_average.pdf} 
    %%for now \caption{2D Pt $R=0.4$ (left), $R=1.0$ (right).}
    \end{figure}
    
    %%% Mass %%%
    \begin{figure}[h!]
    \centering
    \includegraphics[width=8cm]{./figures/angs2D_filter_herwig_average/2D_X4Y49Z137_clone_h_no_cut_FastJets04MassLam50__pythia_average.pdf} 
    \includegraphics[width=8cm]{./figures/angs2D_filter_herwig_average/2D_X1Y518Z1325_clone_h_no_cut_FastJets10MassLam50__pythia_average.pdf} 
    \caption{Quark and Gluon averaged angularities $\lambda_{2}^{1}$ - left R = 0.4, right R = 1.0. 
    Using \pythia{} event generator, at Q50 region, using average of 6 energy combinations 
    900-2360, 900-7000, 900-13000, 2360-7000, 2360-13000, 7000-13000~GeV.}
    \label{fig:Q50_2D_mass2_pyt}
    %%for now \includegraphics[width=8cm]{./figures/angs2D_filter_herwig_average/2D_7_clone_h_no_cut_FastJets04MassLam50__pythia_average.pdf} 
    %%for now \includegraphics[width=8cm]{./figures/angs2D_filter_herwig_average/2D_3_clone_h_no_cut_FastJets10MassLam50__pythia_average.pdf} 
    %%for now \caption{2D Mass $R=0.4$ (left), $R=1.0$ (right).}
    \end{figure}
    \clearpage

    \subsection{\herwig{} 1D Approach, Six Enerrgy Variations, Q50, Trimmed Jets}
    \begin{itemize}
        \item 5 - angularities $\lambda_0^0$, $\lambda_{0.5}^1$, $\lambda_1^1$, $\lambda_0^2$, $\lambda_2^1$ 
        \item 2 - quark/gluon
        \item 1 - using trimmed jets 
        \item 2 - jet radii $R = 0.4, 1.0$
        \item 1 - average of 6 energy combinations: 900-2360, 900-7000, 900-13000, 2360-7000, 2360-13000, 7000-13000~GeV
        \item 1 - event generators \herwig{}
        \item 1 - region - dijet average $p_{T}$ cut (Q50)
        \item 2 - MPI and ISR switched on/off
        \item 1 - gluon fraction $f(p_{T})$ 1D approach
    \end{itemize}

    %%% Multiplicity %%%
    \begin{figure}[h!]
        \centering
        \includegraphics[width=8cm]{./figures/angs1D_filter_herwig_average/1D_X20Y23Z83W27T117R32_clone_h_no_cut_mmdt_FastJets04MultLam50__herwig_average.pdf} 
        \includegraphics[width=8cm]{./figures/angs1D_filter_herwig_average/1D_X3Y167Z218W54T32R25_clone_h_no_cut_mmdt_FastJets10MultLam50__herwig_average.pdf} 
        \caption{Quark and Gluon averaged angularities $\lambda_{0}^{0}$ - left R = 0.4, right R = 1.0. 
        Using \herwig{} event generator, at Q50 region, using average of 6 energy combinations 
        900-2360, 900-7000, 900-13000, 2360-7000, 2360-13000, 7000-13000~GeV.}
        \label{fig:Q50_mmdt_mult2}
        %%for now \includegraphics[width=8cm]{./figures/angs2D_filter_herwig_average/2D_17_clone_h_no_cut_mmdt_FastJets04MultLam50__herwig_average.pdf} 
        %%for now \includegraphics[width=8cm]{./figures/angs2D_filter_herwig_average/2D_5_clone_h_no_cut_mmdt_FastJets10MultLam50__herwig_average.pdf} 
        %%for now \caption{2D Multiplicity $R=0.4$ (left), $R=1.0$ (right).}
        \end{figure}
        
        %%% Lha %%%
        \begin{figure}[h!]
        \centering
        \includegraphics[width=8cm]{./figures/angs1D_filter_herwig_average/1D_X6Y16Z72W15T94R20_clone_h_no_cut_mmdt_FastJets04LhaLam50__herwig_average.pdf} 
        \includegraphics[width=8cm]{./figures/angs1D_filter_herwig_average/1D_X2Y200Z314W50T25R16_clone_h_no_cut_mmdt_FastJets10LhaLam50__herwig_average.pdf} 
        \caption{Quark and Gluon averaged angularities $\lambda_{0.5}^{1}$ - left R = 0.4, right R = 1.0. 
        Using \herwig{} event generator, at Q50 region, using average of 6 energy combinations 
        900-2360, 900-7000, 900-13000, 2360-7000, 2360-13000, 7000-13000~GeV.}
        \label{fig:Q50_mmdt_lha2}
    
        %%for now \includegraphics[width=8cm]{./figures/angs2D_filter_herwig_average/2D_13_clone_h_no_cut_mmdt_FastJets04LhaLam50__herwig_average.pdf} 
        %%for now \includegraphics[width=8cm]{./figures/angs2D_filter_herwig_average/2D_5_clone_h_no_cut_mmdt_FastJets10LhaLam50__herwig_average.pdf} 
        %%for now \caption{2D Lha $R=0.4$ (left), $R=1.0$ (right).}
        \end{figure}
        
        %%% Width %%%
        \begin{figure}[h!]
        \centering
        \includegraphics[width=8cm]{./figures/angs1D_filter_herwig_average/1D_X5Y23Z112W13T59R12_clone_h_no_cut_mmdt_FastJets04WidthLam50__herwig_average.pdf} 
        \includegraphics[width=8cm]{./figures/angs1D_filter_herwig_average/1D_X2Y167Z242W52T31R21_clone_h_no_cut_mmdt_FastJets10WidthLam50__herwig_average.pdf} 
        \caption{Quark and Gluon averaged angularities $\lambda_{1}^{1}$ - left R = 0.4, right R = 1.0. 
        Using \herwig{} event generator, at Q50 region, using average of 6 energy combinations 
        900-2360, 900-7000, 900-13000, 2360-7000, 2360-13000, 7000-13000~GeV.}
        \label{fig:Q50_mmdt_width2}
    
        %%for now \includegraphics[width=8cm]{./figures/angs2D_filter_herwig_average/2D_11_clone_h_no_cut_mmdt_FastJets04WidthLam50__herwig_average.pdf} 
        %%for now \includegraphics[width=8cm]{./figures/angs2D_filter_herwig_average/2D_4_clone_h_no_cut_mmdt_FastJets10WidthLam50__herwig_average.pdf} 
        %%for now \caption{2D Width $R=0.4$ (left), $R=1.0$ (right).}
        \end{figure}
        
        %%% Pt %%%
        \begin{figure}[h!]
        \centering
        \includegraphics[width=8cm]{./figures/angs1D_filter_herwig_average/1D_X15Y11Z71W20T189R29_clone_h_no_cut_mmdt_FastJets04PtLam50__herwig_average.pdf} 
        \includegraphics[width=8cm]{./figures/angs1D_filter_herwig_average/1D_X3Y157Z321W44T28R14_clone_h_no_cut_mmdt_FastJets10PtLam50__herwig_average.pdf} 
        \caption{Quark and Gluon averaged angularities $\lambda_{0}^{2}$ - left R = 0.4, right R = 1.0. 
        Using \herwig{} event generator, at Q50 region, using average of 6 energy combinations 
        900-2360, 900-7000, 900-13000, 2360-7000, 2360-13000, 7000-13000~GeV.}
        \label{fig:Q50_mmdt_pt2}
        %%for now \includegraphics[width=8cm]{./figures/angs2D_filter_herwig_average/2D_42_clone_h_no_cut_mmdt_FastJets04PtLam50__herwig_average.pdf} 
        %%for now \includegraphics[width=8cm]{./figures/angs2D_filter_herwig_average/2D_11_clone_h_no_cut_mmdt_FastJets10PtLam50__herwig_average.pdf} 
        %%for now \caption{2D Pt $R=0.4$ (left), $R=1.0$ (right).}
        \end{figure}
        
        %%% Mass %%%
        \begin{figure}[h!]
        \centering
        \includegraphics[width=8cm]{./figures/angs1D_filter_herwig_average/1D_X4Y19Z90W12T65R13_clone_h_no_cut_mmdt_FastJets04MassLam50__herwig_average.pdf} 
        \includegraphics[width=8cm]{./figures/angs1D_filter_herwig_average/1D_X2Y133Z216W52T39R24_clone_h_no_cut_mmdt_FastJets10MassLam50__herwig_average.pdf} 
        \caption{Quark and Gluon averaged angularities $\lambda_{2}^{1}$ - left R = 0.4, right R = 1.0. 
        Using \herwig{} event generator, at Q50 region, using average of 6 energy combinations 
        900-2360, 900-7000, 900-13000, 2360-7000, 2360-13000, 7000-13000~GeV.}
        \label{fig:Q50_mmdt_mass2}
        %%for now \includegraphics[width=8cm]{./figures/angs2D_filter_herwig_average/2D_14_clone_h_no_cut_mmdt_FastJets04MassLam50__herwig_average.pdf} 
        %%for now \includegraphics[width=8cm]{./figures/angs2D_filter_herwig_average/2D_X2Y90Z145_clone_h_no_cut_mmdt_FastJets10MassLam50__herwig_average.pdf} 
        %%for now \caption{2D Mass $R=0.4$ (left), $R=1.0$ (right).}
        \end{figure}
        \clearpage
    %%%%%%%%%%%%%%%%%%PYTHIA RESULTS %%%%%%%%%%%%%%%%%%%%%%%%%%%%%%%%%%
    \subsection{\pythia{} 1D Approach, Six Enerrgy Variations, Q50, Trimmed Jets}
    \begin{itemize}
        \item 5 - angularities $\lambda_0^0$, $\lambda_{0.5}^1$, $\lambda_1^1$, $\lambda_0^2$, $\lambda_2^1$ 
        \item 2 - quark/gluon
        \item 1 - using trimmed jets 
        \item 2 - jet radii $R = 0.4, 1.0$
        \item 1 - average of 6 energy combinations: 900-2360, 900-7000, 900-13000, 2360-7000, 2360-13000, 7000-13000~GeV
        \item 1 - event generators \pythia{}
        \item 1 - region - dijet average $p_{T}$ cut (Q50)
        \item 2 - MPI and ISR switched on/off
        \item 1 - gluon fraction $f(p_{T})$ 1D approach
    \end{itemize}

    %%% Multiplicity %%%
    \begin{figure}[h!]
        \centering
        \includegraphics[width=8cm]{./figures/angs1D_filter_herwig_average/1D_X6Y136Z443W28T21R6_clone_h_no_cut_mmdt_FastJets04MultLam50__pythia_average.pdf} 
        \includegraphics[width=8cm]{./figures/angs1D_filter_herwig_average/1D_X1Y642Z859W61T10R7_clone_h_no_cut_mmdt_FastJets10MultLam50__pythia_average.pdf} 
        \caption{Quark and Gluon averaged angularities $\lambda_{0}^{0}$ - left R = 0.4, right R = 1.0. 
        Using \pythia{} event generator, at Q50 region, using average of 6 energy combinations 
        900-2360, 900-7000, 900-13000, 2360-7000, 2360-13000, 7000-13000~GeV.}
        \label{fig:Q50_mmdt_mult2_pyt}
        %%for now \includegraphics[width=8cm]{./figures/angs2D_filter_herwig_average/2D_17_clone_h_no_cut_mmdt_FastJets04MultLam50__pythia_average.pdf} 
        %%for now \includegraphics[width=8cm]{./figures/angs2D_filter_herwig_average/2D_5_clone_h_no_cut_mmdt_FastJets10MultLam50__pythia_average.pdf} 
        %%for now \caption{2D Multiplicity $R=0.4$ (left), $R=1.0$ (right).}
        \end{figure}
        
        %%% Lha %%%
        \begin{figure}[h!]
        \centering
        \includegraphics[width=8cm]{./figures/angs1D_filter_herwig_average/1D_X6Y51Z342W14T28R4_clone_h_no_cut_mmdt_FastJets04LhaLam50__pythia_average.pdf} 
        \includegraphics[width=8cm]{./figures/angs1D_filter_herwig_average/1D_X1Y310Z423W58T19R14_clone_h_no_cut_mmdt_FastJets10LhaLam50__pythia_average.pdf} 
        \caption{Quark and Gluon averaged angularities $\lambda_{0.5}^{1}$ - left R = 0.4, right R = 1.0. 
        Using \pythia{} event generator, at Q50 region, using average of 6 energy combinations 
        900-2360, 900-7000, 900-13000, 2360-7000, 2360-13000, 7000-13000~GeV.}
        \label{fig:Q50_mmdt_lha2_pyt}
    
        %%for now \includegraphics[width=8cm]{./figures/angs2D_filter_herwig_average/2D_13_clone_h_no_cut_mmdt_FastJets04LhaLam50__pythia_average.pdf} 
        %%for now \includegraphics[width=8cm]{./figures/angs2D_filter_herwig_average/2D_5_clone_h_no_cut_mmdt_FastJets10LhaLam50__pythia_average.pdf} 
        %%for now \caption{2D Lha $R=0.4$ (left), $R=1.0$ (right).}
        \end{figure}
        
        %%% Width %%%
        \begin{figure}[h!]
        \centering
        \includegraphics[width=8cm]{./figures/angs1D_filter_herwig_average/1D_X5Y51Z287W13T25R4_clone_h_no_cut_mmdt_FastJets04WidthLam50__pythia_average.pdf} 
        \includegraphics[width=8cm]{./figures/angs1D_filter_herwig_average/1D_X1Y294Z392W60T21R15_clone_h_no_cut_mmdt_FastJets10WidthLam50__pythia_average.pdf} 
        \caption{Quark and Gluon averaged angularities $\lambda_{1}^{1}$ - left R = 0.4, right R = 1.0. 
        Using \pythia{} event generator, at Q50 region, using average of 6 energy combinations 
        900-2360, 900-7000, 900-13000, 2360-7000, 2360-13000, 7000-13000~GeV.}
        \label{fig:Q50_mmdt_width2_pyt}
    
        %%for now \includegraphics[width=8cm]{./figures/angs2D_filter_herwig_average/2D_11_clone_h_no_cut_mmdt_FastJets04WidthLam50__pythia_average.pdf} 
        %%for now \includegraphics[width=8cm]{./figures/angs2D_filter_herwig_average/2D_4_clone_h_no_cut_mmdt_FastJets10WidthLam50__pythia_average.pdf} 
        %%for now \caption{2D Width $R=0.4$ (left), $R=1.0$ (right).}
        \end{figure}
        
        %%% Pt %%%
        \begin{figure}[h!]
        \centering
        \includegraphics[width=8cm]{./figures/angs1D_filter_herwig_average/1D_X14Y30Z98W22T71R22_clone_h_no_cut_mmdt_FastJets04PtLam50__pythia_average.pdf} 
        \includegraphics[width=8cm]{./figures/angs1D_filter_herwig_average/1D_X2Y228Z374W51T22R14_clone_h_no_cut_mmdt_FastJets10PtLam50__pythia_average.pdf} 
        \caption{Quark and Gluon averaged angularities $\lambda_{0}^{2}$ - left R = 0.4, right R = 1.0. 
        Using \pythia{} event generator, at Q50 region, using average of 6 energy combinations 
        900-2360, 900-7000, 900-13000, 2360-7000, 2360-13000, 7000-13000~GeV.}
        \label{fig:Q50_mmdt_pt2_pyt}
        %%for now \includegraphics[width=8cm]{./figures/angs2D_filter_herwig_average/2D_42_clone_h_no_cut_mmdt_FastJets04PtLam50__pythia_average.pdf} 
        %%for now \includegraphics[width=8cm]{./figures/angs2D_filter_herwig_average/2D_11_clone_h_no_cut_mmdt_FastJets10PtLam50__pythia_average.pdf} 
        %%for now \caption{2D Pt $R=0.4$ (left), $R=1.0$ (right).}
        \end{figure}
        
        %%% Mass %%%
        \begin{figure}[h!]
        \centering
        \includegraphics[width=8cm]{./figures/angs1D_filter_herwig_average/1D_X4Y42Z199W12T29R6_clone_h_no_cut_mmdt_FastJets04MassLam50__pythia_average.pdf} 
        \includegraphics[width=8cm]{./figures/angs1D_filter_herwig_average/1D_X1Y260Z336W62T24R18_clone_h_no_cut_mmdt_FastJets10MassLam50__pythia_average.pdf} 
        \caption{Quark and Gluon averaged angularities $\lambda_{2}^{1}$ - left R = 0.4, right R = 1.0. 
        Using \pythia{} event generator, at Q50 region, using average of 6 energy combinations 
        900-2360, 900-7000, 900-13000, 2360-7000, 2360-13000, 7000-13000~GeV.}
        \label{fig:Q50_mmdt_mass2_pyt}
        %%for now \includegraphics[width=8cm]{./figures/angs2D_filter_herwig_average/2D_7_clone_h_no_cut_mmdt_FastJets04MassLam50__pythia_average.pdf} 
        %%for now \includegraphics[width=8cm]{./figures/angs2D_filter_herwig_average/2D_3_clone_h_no_cut_mmdt_FastJets10MassLam50__pythia_average.pdf} 
        %%for now \caption{2D Mass $R=0.4$ (left), $R=1.0$ (right).}
        \end{figure}
        \clearpage
    %%%% 2D APPROACH%%%%%%%%%%%%%%%%%%%%%%%%%%%
    \subsection{\herwig{} 2D Approach, Six Enerrgy Variations, Q50, Trimmed Jets}
    \begin{itemize}
        \item 5 - angularities $\lambda_0^0$, $\lambda_{0.5}^1$, $\lambda_1^1$, $\lambda_0^2$, $\lambda_2^1$ 
        \item 2 - quark/gluon
        \item 1 - using trimmed jets 
        \item 2 - jet radii $R = 0.4, 1.0$
        \item 1 - average of 6 energy combinations: 900-2360, 900-7000, 900-13000, 2360-7000, 2360-13000, 7000-13000~GeV
        \item 1 - event generators \herwig{}
        \item 1 - region - dijet average $p_{T}$ cut (Q50)
        \item 2 - MPI and ISR switched on/off
        \item 1 - gluon fraction $f(p_{T})$ 2D approach
    \end{itemize}

    %%% Multiplicity %%%
    \begin{figure}[h!]
        \centering
        \includegraphics[width=8cm]{./figures/angs2D_filter_herwig_average/2D_X15Y17Z45_clone_h_no_cut_mmdt_FastJets04MultLam50__herwig_average.pdf} 
        \includegraphics[width=8cm]{./figures/angs2D_filter_herwig_average/2D_X3Y98Z139_clone_h_no_cut_mmdt_FastJets10MultLam50__herwig_average.pdf} 
        \caption{Quark and Gluon averaged angularities $\lambda_{0}^{0}$ - left R = 0.4, right R = 1.0. 
        Using \herwig{} event generator, at Q50 region, using average of 6 energy combinations 
        900-2360, 900-7000, 900-13000, 2360-7000, 2360-13000, 7000-13000~GeV.}
        \label{fig:Q50_mmdt_2D_mult2}
        %%for now \includegraphics[width=8cm]{./figures/angs2D_filter_herwig_average/2D_17_clone_h_no_cut_mmdt_FastJets04MultLam50__herwig_average.pdf} 
        %%for now \includegraphics[width=8cm]{./figures/angs2D_filter_herwig_average/2D_5_clone_h_no_cut_mmdt_FastJets10MultLam50__herwig_average.pdf} 
        %%for now \caption{2D Multiplicity $R=0.4$ (left), $R=1.0$ (right).}
        \end{figure}
        
        %%% Lha %%%
        \begin{figure}[h!]
        \centering
        \includegraphics[width=8cm]{./figures/angs2D_filter_herwig_average/2D_X5Y13Z54_clone_h_no_cut_mmdt_FastJets04LhaLam50__herwig_average.pdf} 
        \includegraphics[width=8cm]{./figures/angs2D_filter_herwig_average/2D_X2Y122Z168_clone_h_no_cut_mmdt_FastJets10LhaLam50__herwig_average.pdf} 
        \caption{Quark and Gluon averaged angularities $\lambda_{0.5}^{1}$ - left R = 0.4, right R = 1.0. 
        Using \herwig{} event generator, at Q50 region, using average of 6 energy combinations 
        900-2360, 900-7000, 900-13000, 2360-7000, 2360-13000, 7000-13000~GeV.}
        \label{fig:Q50_mmdt_2D_lha2}
    
        %%for now \includegraphics[width=8cm]{./figures/angs2D_filter_herwig_average/2D_13_clone_h_no_cut_mmdt_FastJets04LhaLam50__herwig_average.pdf} 
        %%for now \includegraphics[width=8cm]{./figures/angs2D_filter_herwig_average/2D_5_clone_h_no_cut_mmdt_FastJets10LhaLam50__herwig_average.pdf} 
        %%for now \caption{2D Lha $R=0.4$ (left), $R=1.0$ (right).}
        \end{figure}
        
        %%% Width %%%
        \begin{figure}[h!]
        \centering
        \includegraphics[width=8cm]{./figures/angs2D_filter_herwig_average/2D_X4Y18Z113_clone_h_no_cut_mmdt_FastJets04WidthLam50__herwig_average.pdf} 
        \includegraphics[width=8cm]{./figures/angs2D_filter_herwig_average/2D_X2Y108Z339_clone_h_no_cut_mmdt_FastJets10WidthLam50__herwig_average.pdf} 
        \caption{Quark and Gluon averaged angularities $\lambda_{1}^{1}$ - left R = 0.4, right R = 1.0. 
        Using \herwig{} event generator, at Q50 region, using average of 6 energy combinations 
        900-2360, 900-7000, 900-13000, 2360-7000, 2360-13000, 7000-13000~GeV.}
        \label{fig:Q50_mmdt_2D_width2}
    
        %%for now \includegraphics[width=8cm]{./figures/angs2D_filter_herwig_average/2D_11_clone_h_no_cut_mmdt_FastJets04WidthLam50__herwig_average.pdf} 
        %%for now \includegraphics[width=8cm]{./figures/angs2D_filter_herwig_average/2D_4_clone_h_no_cut_mmdt_FastJets10WidthLam50__herwig_average.pdf} 
        %%for now \caption{2D Width $R=0.4$ (left), $R=1.0$ (right).}
        \end{figure}
        
        %%% Pt %%%
        \begin{figure}[h!]
        \centering
        \includegraphics[width=8cm]{./figures/angs2D_filter_herwig_average/2D_X10Y8Z35_clone_h_no_cut_mmdt_FastJets04PtLam50__herwig_average.pdf} 
        \includegraphics[width=8cm]{./figures/angs2D_filter_herwig_average/2D_X3Y80Z152_clone_h_no_cut_mmdt_FastJets10PtLam50__herwig_average.pdf} 
        \caption{Quark and Gluon averaged angularities $\lambda_{0}^{2}$ - left R = 0.4, right R = 1.0. 
        Using \herwig{} event generator, at Q50 region, using average of 6 energy combinations 
        900-2360, 900-7000, 900-13000, 2360-7000, 2360-13000, 7000-13000~GeV.}
        \label{fig:Q50_mmdt_2D_pt2}
        %%for now \includegraphics[width=8cm]{./figures/angs2D_filter_herwig_average/2D_42_clone_h_no_cut_mmdt_FastJets04PtLam50__herwig_average.pdf} 
        %%for now \includegraphics[width=8cm]{./figures/angs2D_filter_herwig_average/2D_11_clone_h_no_cut_mmdt_FastJets10PtLam50__herwig_average.pdf} 
        %%for now \caption{2D Pt $R=0.4$ (left), $R=1.0$ (right).}
        \end{figure}
        
        %%% Mass %%%
        \begin{figure}[h!]
        \centering
        \includegraphics[width=8cm]{./figures/angs2D_filter_herwig_average/2D_X4Y14Z81_clone_h_no_cut_mmdt_FastJets04MassLam50__herwig_average.pdf} 
        \includegraphics[width=8cm]{./figures/angs2D_filter_herwig_average/2D_X2Y90Z145_clone_h_no_cut_mmdt_FastJets10MassLam50__herwig_average.pdf} 
        \caption{Quark and Gluon averaged angularities $\lambda_{2}^{1}$ - left R = 0.4, right R = 1.0. 
        Using \herwig{} event generator, at Q50 region, using average of 6 energy combinations 
        900-2360, 900-7000, 900-13000, 2360-7000, 2360-13000, 7000-13000~GeV.}
        \label{fig:Q50_mmdt_2D_mass2}
        %%for now \includegraphics[width=8cm]{./figures/angs2D_filter_herwig_average/2D_7_clone_h_no_cut_mmdt_FastJets04MassLam50__herwig_average.pdf} 
        %%for now \includegraphics[width=8cm]{./figures/angs2D_filter_herwig_average/2D_3_clone_h_no_cut_mmdt_FastJets10MassLam50__herwig_average.pdf} 
        %%for now \caption{2D Mass $R=0.4$ (left), $R=1.0$ (right).}
        \end{figure}
        \clearpage
    %%%%%%%%%%%%%%%%%%PYTHIA RESULTS %%%%%%%%%%%%%%%%%%%%%%%%%%%%%%%%%%
    \subsection{\pythia{} 2D Approach, Six Enerrgy Variations, Q50, Trimmed Jets}
    \begin{itemize}
        \item 5 - angularities $\lambda_0^0$, $\lambda_{0.5}^1$, $\lambda_1^1$, $\lambda_0^2$, $\lambda_2^1$ 
        \item 2 - quark/gluon
        \item 1 - using trimmed jets 
        \item 2 - jet radii $R = 0.4, 1.0$
        \item 1 - average of 6 energy combinations: 900-2360, 900-7000, 900-13000, 2360-7000, 2360-13000, 7000-13000~GeV
        \item 1 - event generators \pythia{}
        \item 1 - region - dijet average $p_{T}$ cut (Q50)
        \item 2 - MPI and ISR switched on/off
        \item 1 - gluon fraction $f(p_{T})$ 2D approach
    \end{itemize}

    %%% Multiplicity %%%
    \begin{figure}[h!]
        \centering
        \includegraphics[width=8cm]{./figures/angs2D_filter_herwig_average/2D_X6Y60Z140_clone_h_no_cut_mmdt_FastJets04MultLam50__pythia_average.pdf} 
        \includegraphics[width=8cm]{./figures/angs2D_filter_herwig_average/2D_X1Y299Z319_clone_h_no_cut_mmdt_FastJets10MultLam50__pythia_average.pdf} 
        \caption{Quark and Gluon averaged angularities $\lambda_{0}^{0}$ - left R = 0.4, right R = 1.0. 
        Using \pythia{} event generator, at Q50 region, using average of 6 energy combinations 
        900-2360, 900-7000, 900-13000, 2360-7000, 2360-13000, 7000-13000~GeV.}
        \label{fig:Q50_mmdt_2D_mult2_pyt}
        %%for now \includegraphics[width=8cm]{./figures/angs2D_filter_herwig_average/2D_17_clone_h_no_cut_mmdt_FastJets04MultLam50__pythia_average.pdf} 
        %%for now \includegraphics[width=8cm]{./figures/angs2D_filter_herwig_average/2D_5_clone_h_no_cut_mmdt_FastJets10MultLam50__pythia_average.pdf} 
        %%for now \caption{2D Multiplicity $R=0.4$ (left), $R=1.0$ (right).}
        \end{figure}
        
        %%% Lha %%%
        \begin{figure}[h!]
        \centering
        \includegraphics[width=8cm]{./figures/angs2D_filter_herwig_average/2D_X6Y28Z151_clone_h_no_cut_mmdt_FastJets04LhaLam50__pythia_average.pdf} 
        \includegraphics[width=8cm]{./figures/angs2D_filter_herwig_average/2D_X1Y225Z272_clone_h_no_cut_mmdt_FastJets10LhaLam50__pythia_average.pdf} 
        \caption{Quark and Gluon averaged angularities $\lambda_{0.5}^{1}$ - left R = 0.4, right R = 1.0. 
        Using \pythia{} event generator, at Q50 region, using average of 6 energy combinations 
        900-2360, 900-7000, 900-13000, 2360-7000, 2360-13000, 7000-13000~GeV.}
        \label{fig:Q50_mmdt_2D_lha2_pyt}
    
        %%for now \includegraphics[width=8cm]{./figures/angs2D_filter_herwig_average/2D_13_clone_h_no_cut_mmdt_FastJets04LhaLam50__pythia_average.pdf} 
        %%for now \includegraphics[width=8cm]{./figures/angs2D_filter_herwig_average/2D_5_clone_h_no_cut_mmdt_FastJets10LhaLam50__pythia_average.pdf} 
        %%for now \caption{2D Lha $R=0.4$ (left), $R=1.0$ (right).}
        \end{figure}
        
        %%% Width %%%
        \begin{figure}[h!]
        \centering
        \includegraphics[width=8cm]{./figures/angs2D_filter_herwig_average/2D_X4Y27Z102_clone_h_no_cut_mmdt_FastJets04WidthLam50__pythia_average.pdf} 
        \includegraphics[width=8cm]{./figures/angs2D_filter_herwig_average/2D_X1Y209Z248_clone_h_no_cut_mmdt_FastJets10WidthLam50__pythia_average.pdf} 
        \caption{Quark and Gluon averaged angularities $\lambda_{1}^{1}$ - left R = 0.4, right R = 1.0. 
        Using \pythia{} event generator, at Q50 region, using average of 6 energy combinations 
        900-2360, 900-7000, 900-13000, 2360-7000, 2360-13000, 7000-13000~GeV.}
        \label{fig:Q50_mmdt_2D_width2_pyt}
    
        %%for now \includegraphics[width=8cm]{./figures/angs2D_filter_herwig_average/2D_11_clone_h_no_cut_mmdt_FastJets04WidthLam50__pythia_average.pdf} 
        %%for now \includegraphics[width=8cm]{./figures/angs2D_filter_herwig_average/2D_4_clone_h_no_cut_mmdt_FastJets10WidthLam50__pythia_average.pdf} 
        %%for now \caption{2D Width $R=0.4$ (left), $R=1.0$ (right).}
        \end{figure}
        
        %%% Pt %%%
        \begin{figure}[h!]
        \centering
        \includegraphics[width=8cm]{./figures/angs2D_filter_herwig_average/2D_X13Y18Z62_clone_h_no_cut_mmdt_FastJets04PtLam50__pythia_average.pdf} 
        \includegraphics[width=8cm]{./figures/angs2D_filter_herwig_average/2D_X1Y123Z155_clone_h_no_cut_mmdt_FastJets10PtLam50__pythia_average.pdf} 
        \caption{Quark and Gluon averaged angularities $\lambda_{0}^{2}$ - left R = 0.4, right R = 1.0. 
        Using \pythia{} event generator, at Q50 region, using average of 6 energy combinations 
        900-2360, 900-7000, 900-13000, 2360-7000, 2360-13000, 7000-13000~GeV.}
        \label{fig:Q50_mmdt_2D_pt2_pyt}
        %%for now \includegraphics[width=8cm]{./figures/angs2D_filter_herwig_average/2D_42_clone_h_no_cut_mmdt_FastJets04PtLam50__pythia_average.pdf} 
        %%for now \includegraphics[width=8cm]{./figures/angs2D_filter_herwig_average/2D_11_clone_h_no_cut_mmdt_FastJets10PtLam50__pythia_average.pdf} 
        %%for now \caption{2D Pt $R=0.4$ (left), $R=1.0$ (right).}
        \end{figure}
        
        %%% Mass %%%
        \begin{figure}[h!]
        \centering
        \includegraphics[width=8cm]{./figures/angs2D_filter_herwig_average/2D_X4Y25Z96_clone_h_no_cut_mmdt_FastJets04MassLam50__pythia_average.pdf} 
        \includegraphics[width=8cm]{./figures/angs2D_filter_herwig_average/2D_X1Y175Z235_clone_h_no_cut_mmdt_FastJets10MassLam50__pythia_average.pdf} 
        \caption{Quark and Gluon averaged angularities $\lambda_{2}^{1}$ - left R = 0.4, right R = 1.0. 
        Using \pythia{} event generator, at Q50 region, using average of 6 energy combinations 
        900-2360, 900-7000, 900-13000, 2360-7000, 2360-13000, 7000-13000~GeV.}
        \label{fig:Q50_mmdt_2D_mass2_pyt}
        %%for now \includegraphics[width=8cm]{./figures/angs2D_filter_herwig_average/2D_7_clone_h_no_cut_mmdt_FastJets04MassLam50__pythia_average.pdf} 
        %%for now \includegraphics[width=8cm]{./figures/angs2D_filter_herwig_average/2D_3_clone_h_no_cut_mmdt_FastJets10MassLam50__pythia_average.pdf} 
        %%for now \caption{2D Mass $R=0.4$ (left), $R=1.0$ (right).}
        \end{figure}
        \clearpage
